# Supplementary material for: AMLB: an AutoML Benchmark
Source: arXiv:2207.12560 source file (2023-11-16)
Supplement: Supplementary file 1 [file auc-1h8c_gp3-table.tex]

\footnotesize
\begin{landscape}
\begin{table}
\tiny
\begin{tabular}{rlrrrrrrrrr}
\toprule
 & framework& \unsizedsystemcase{autogluon}\ \ \  & \unsizedsystemcase{auto-sklearn}\ \ \  & \unsizedsystemcase{auto-sklearn 2} & \unsizedsystemcase{flaml}\ \ \ & \unsizedsystemcase{gama}\ \ \ & \unsizedsystemcase{h2o automl}\ \ \  & \unsizedsystemcase{light automl}\ \ \  & \unsizedsystemcase{mljar}\ \ \  & \unsizedsystemcase{tpot}\ \ \  \\
 task id & task name & & & & & & & & & \\
\midrule
146818 & australi... & 0.941(0.019)$^{\hspace{0.4em}}$ & 0.932(0.020)$^{\hspace{0.4em}}$ & 0.937(0.020)$^{\hspace{0.4em}}$ & 0.942(0.017)$^{\hspace{0.4em}}$ & 0.941(0.019)$^{\hspace{0.4em}}$ & 0.934(0.024)$^{\hspace{0.4em}}$ & 0.944(0.022)$^{\hspace{0.4em}}$ & 0.945(0.018)$^{\hspace{0.4em}}$ & 0.937(0.021)$^{\hspace{0.4em}}$ \\
146820 & wilt & 0.994(0.010)$^{\hspace{0.4em}}$ & 0.997(0.003)$^{\hspace{0.4em}}$ & 0.994(0.008)$^{\hspace{0.4em}}$ & 0.992(0.012)$^{\hspace{0.4em}}$ & 0.995(0.005)$^{\hspace{0.4em}}$ & 0.994(0.007)$^{\hspace{0.4em}}$ & 0.994(0.007)$^{\hspace{0.4em}}$ & 0.996(0.004)$^{4}$ & 0.994(0.007)$^{\hspace{0.4em}}$ \\
167120 & numerai2... & 0.525(0.005)$^{\hspace{0.4em}}$ & 0.529(0.005)$^{\hspace{0.4em}}$ & 0.530(0.004)$^{\hspace{0.4em}}$ & 0.528(0.004)$^{\hspace{0.4em}}$ & 0.531(0.004)$^{\hspace{0.4em}}$ & 0.532(0.005)$^{\hspace{0.4em}}$ & 0.531(0.005)$^{\hspace{0.4em}}$ & 0.530(0.004)$^{\hspace{0.4em}}$ & 0.527(0.006)$^{\hspace{0.4em}}$ \\
168350 & phoneme & 0.972(0.008)$^{\hspace{0.4em}}$ & 0.965(0.009)$^{\hspace{0.4em}}$ & 0.970(0.008)$^{\hspace{0.4em}}$ & 0.972(0.010)$^{\hspace{0.4em}}$ & 0.971(0.009)$^{\hspace{0.4em}}$ & 0.967(0.009)$^{\hspace{0.4em}}$ & 0.965(0.008)$^{\hspace{0.4em}}$ & 0.976(0.004)$^{7}$ & 0.969(0.010)$^{\hspace{0.4em}}$ \\
168757 & credit-g & 0.791(0.042)$^{\hspace{0.4em}}$ & 0.777(0.049)$^{\hspace{0.4em}}$ & 0.797(0.037)$^{\hspace{0.4em}}$ & 0.780(0.045)$^{\hspace{0.4em}}$ & 0.794(0.028)$^{\hspace{0.4em}}$ & 0.798(0.033)$^{\hspace{0.4em}}$ & 0.791(0.037)$^{\hspace{0.4em}}$ & -$\hspace{0.4em}$ & 0.791(0.039)$^{\hspace{0.4em}}$ \\
168868 & apsfailu... & 0.992(0.003)$^{\hspace{0.4em}}$ & 0.992(0.003)$^{\hspace{0.4em}}$ & 0.992(0.002)$^{\hspace{0.4em}}$ & 0.991(0.003)$^{\hspace{0.4em}}$ & 0.990(0.003)$^{\hspace{0.4em}}$ & 0.992(0.002)$^{\hspace{0.4em}}$ & 0.992(0.002)$^{5}$ & 0.993(0.002)$^{1}$ & 0.990(0.003)$^{\hspace{0.4em}}$ \\
168911 & jasmine & 0.887(0.017)$^{\hspace{0.4em}}$ & 0.884(0.017)$^{\hspace{0.4em}}$ & 0.887(0.016)$^{\hspace{0.4em}}$ & 0.885(0.018)$^{\hspace{0.4em}}$ & 0.894(0.016)$^{\hspace{0.4em}}$ & 0.884(0.018)$^{\hspace{0.4em}}$ & 0.880(0.018)$^{\hspace{0.4em}}$ & 0.887(0.016)$^{\hspace{0.4em}}$ & 0.886(0.015)$^{\hspace{0.4em}}$ \\
189354 & airlines & 0.728(0.002)$^{\hspace{0.4em}}$ & 0.726(0.002)$^{\hspace{0.4em}}$ & 0.728(0.002)$^{\hspace{0.4em}}$ & 0.731(0.002)$^{\hspace{0.4em}}$ & 0.724(0.005)$^{\hspace{0.4em}}$ & 0.731(0.002)$^{\hspace{0.4em}}$ & 0.728(0.002)$^{\hspace{0.4em}}$ & 0.730(0.002)$^{\hspace{0.4em}}$ & 0.724(0.002)$^{\hspace{0.4em}}$ \\
189356 & albert & 0.781(0.003)$^{\hspace{0.4em}}$ & 0.760(0.004)$^{\hspace{0.4em}}$ & 0.756(0.003)$^{\hspace{0.4em}}$ & 0.778(0.004)$^{\hspace{0.4em}}$ & 0.716(0.012)$^{\hspace{0.4em}}$ & 0.763(0.003)$^{\hspace{0.4em}}$ & 0.782(0.002)$^{\hspace{0.4em}}$ & 0.783(0.002)$^{\hspace{0.4em}}$ & 0.725(0.015)$^{\hspace{0.4em}}$ \\
189922 & gina & 0.992(0.005)$^{\hspace{0.4em}}$ & 0.989(0.007)$^{\hspace{0.4em}}$ & 0.987(0.007)$^{\hspace{0.4em}}$ & 0.992(0.005)$^{\hspace{0.4em}}$ & 0.992(0.003)$^{\hspace{0.4em}}$ & 0.990(0.006)$^{\hspace{0.4em}}$ & 0.990(0.006)$^{\hspace{0.4em}}$ & 0.991(0.005)$^{\hspace{0.4em}}$ & 0.988(0.007)$^{\hspace{0.4em}}$ \\
190137 & ozone-le... & 0.935(0.018)$^{\hspace{0.4em}}$ & 0.920(0.024)$^{\hspace{0.4em}}$ & 0.928(0.024)$^{\hspace{0.4em}}$ & 0.925(0.025)$^{\hspace{0.4em}}$ & 0.924(0.030)$^{\hspace{0.4em}}$ & 0.929(0.018)$^{\hspace{0.4em}}$ & 0.931(0.016)$^{\hspace{0.4em}}$ & 0.930(0.022)$^{3}$ & 0.913(0.037)$^{\hspace{0.4em}}$ \\
190392 & madeline & 0.945(0.009)$^{\hspace{0.4em}}$ & 0.969(0.005)$^{\hspace{0.4em}}$ & 0.944(0.008)$^{\hspace{0.4em}}$ & 0.952(0.011)$^{\hspace{0.4em}}$ & 0.956(0.007)$^{\hspace{0.4em}}$ & 0.944(0.011)$^{\hspace{0.4em}}$ & 0.935(0.008)$^{\hspace{0.4em}}$ & 0.953(0.011)$^{\hspace{0.4em}}$ & 0.948(0.007)$^{\hspace{0.4em}}$ \\
190410 & philippi... & 0.883(0.013)$^{\hspace{0.4em}}$ & 0.911(0.013)$^{\hspace{0.4em}}$ & 0.875(0.014)$^{\hspace{0.4em}}$ & 0.893(0.013)$^{\hspace{0.4em}}$ & 0.895(0.012)$^{\hspace{0.4em}}$ & 0.878(0.012)$^{\hspace{0.4em}}$ & 0.864(0.015)$^{\hspace{0.4em}}$ & 0.881(0.013)$^{\hspace{0.4em}}$ & 0.888(0.014)$^{1}$ \\
190411 & ada & 0.920(0.018)$^{\hspace{0.4em}}$ & 0.919(0.017)$^{\hspace{0.4em}}$ & 0.919(0.018)$^{\hspace{0.4em}}$ & 0.924(0.017)$^{\hspace{0.4em}}$ & 0.920(0.018)$^{\hspace{0.4em}}$ & 0.920(0.018)$^{\hspace{0.4em}}$ & 0.922(0.018)$^{\hspace{0.4em}}$ & 0.920(0.017)$^{\hspace{0.4em}}$ & 0.918(0.018)$^{\hspace{0.4em}}$ \\
190412 & arcene & 0.861(0.170)$^{\hspace{0.4em}}$ & 0.865(0.181)$^{\hspace{0.4em}}$ & 0.845(0.202)$^{\hspace{0.4em}}$ & 0.848(0.204)$^{\hspace{0.4em}}$ & 0.860(0.162)$^{\hspace{0.4em}}$ & 0.853(0.199)$^{\hspace{0.4em}}$ & 0.865(0.133)$^{\hspace{0.4em}}$ & 0.837(0.206)$^{\hspace{0.4em}}$ & 0.853(0.133)$^{4}$ \\
359955 & blood-tr... & 0.752(0.045)$^{\hspace{0.4em}}$ & 0.758(0.045)$^{\hspace{0.4em}}$ & 0.759(0.044)$^{\hspace{0.4em}}$ & 0.734(0.053)$^{\hspace{0.4em}}$ & 0.756(0.048)$^{\hspace{0.4em}}$ & 0.763(0.040)$^{\hspace{0.4em}}$ & 0.748(0.054)$^{\hspace{0.4em}}$ & -$\hspace{0.4em}$ & 0.757(0.055)$^{\hspace{0.4em}}$ \\
359956 & qsar-bio... & 0.942(0.034)$^{\hspace{0.4em}}$ & 0.926(0.033)$^{\hspace{0.4em}}$ & 0.939(0.027)$^{\hspace{0.4em}}$ & 0.930(0.035)$^{\hspace{0.4em}}$ & 0.936(0.032)$^{\hspace{0.4em}}$ & 0.936(0.034)$^{\hspace{0.4em}}$ & 0.933(0.033)$^{\hspace{0.4em}}$ & 0.931(0.036)$^{5}$ & 0.933(0.032)$^{\hspace{0.4em}}$ \\
359958 & pc4 & 0.951(0.018)$^{\hspace{0.4em}}$ & 0.943(0.018)$^{\hspace{0.4em}}$ & 0.948(0.017)$^{\hspace{0.4em}}$ & 0.948(0.021)$^{\hspace{0.4em}}$ & 0.952(0.021)$^{\hspace{0.4em}}$ & 0.947(0.026)$^{\hspace{0.4em}}$ & 0.948(0.016)$^{\hspace{0.4em}}$ & 0.951(0.017)$^{\hspace{0.4em}}$ & 0.951(0.018)$^{\hspace{0.4em}}$ \\
359962 & kc1 & 0.839(0.034)$^{\hspace{0.4em}}$ & 0.842(0.028)$^{\hspace{0.4em}}$ & 0.838(0.035)$^{\hspace{0.4em}}$ & 0.842(0.035)$^{\hspace{0.4em}}$ & 0.849(0.030)$^{\hspace{0.4em}}$ & 0.823(0.042)$^{\hspace{0.4em}}$ & 0.827(0.034)$^{\hspace{0.4em}}$ & 0.828(0.033)$^{\hspace{0.4em}}$ & 0.853(0.036)$^{\hspace{0.4em}}$ \\
359965 & kr-vs-kp & 1.000(0.000)$^{\hspace{0.4em}}$ & 1.000(0.000)$^{\hspace{0.4em}}$ & 1.000(0.000)$^{\hspace{0.4em}}$ & 1.000(0.000)$^{\hspace{0.4em}}$ & 1.000(0.000)$^{\hspace{0.4em}}$ & 1.000(0.001)$^{\hspace{0.4em}}$ & 1.000(0.000)$^{\hspace{0.4em}}$ & 0.999(0.001)$^{\hspace{0.4em}}$ & 0.999(0.001)$^{\hspace{0.4em}}$ \\
359966 & internet... & 0.987(0.009)$^{\hspace{0.4em}}$ & 0.985(0.013)$^{\hspace{0.4em}}$ & 0.986(0.012)$^{\hspace{0.4em}}$ & 0.985(0.011)$^{\hspace{0.4em}}$ & 0.985(0.010)$^{\hspace{0.4em}}$ & 0.986(0.009)$^{\hspace{0.4em}}$ & 0.987(0.010)$^{\hspace{0.4em}}$ & 0.986(0.012)$^{2}$ & 0.984(0.010)$^{\hspace{0.4em}}$ \\
359967 & biorespo... & 0.886(0.016)$^{\hspace{0.4em}}$ & 0.872(0.017)$^{\hspace{0.4em}}$ & 0.872(0.018)$^{\hspace{0.4em}}$ & 0.886(0.016)$^{\hspace{0.4em}}$ & 0.884(0.017)$^{\hspace{0.4em}}$ & 0.886(0.017)$^{\hspace{0.4em}}$ & 0.884(0.017)$^{\hspace{0.4em}}$ & 0.884(0.018)$^{\hspace{0.4em}}$ & 0.879(0.017)$^{\hspace{0.4em}}$ \\
359968 & churn & 0.928(0.024)$^{\hspace{0.4em}}$ & 0.922(0.022)$^{\hspace{0.4em}}$ & 0.920(0.026)$^{\hspace{0.4em}}$ & 0.920(0.018)$^{\hspace{0.4em}}$ & 0.923(0.023)$^{\hspace{0.4em}}$ & 0.922(0.027)$^{\hspace{0.4em}}$ & 0.925(0.021)$^{\hspace{0.4em}}$ & 0.932(0.025)$^{\hspace{0.4em}}$ & 0.918(0.021)$^{\hspace{0.4em}}$ \\
359971 & phishing... & 0.998(0.001)$^{\hspace{0.4em}}$ & 0.997(0.001)$^{\hspace{0.4em}}$ & 0.997(0.001)$^{\hspace{0.4em}}$ & 0.998(0.001)$^{\hspace{0.4em}}$ & 0.997(0.001)$^{\hspace{0.4em}}$ & 0.998(0.001)$^{\hspace{0.4em}}$ & 0.998(0.001)$^{\hspace{0.4em}}$ & 0.998(0.001)$^{5}$ & 0.948(0.157)$^{\hspace{0.4em}}$ \\
359972 & sylvine & 0.991(0.003)$^{\hspace{0.4em}}$ & 0.990(0.004)$^{\hspace{0.4em}}$ & 0.989(0.002)$^{\hspace{0.4em}}$ & 0.991(0.002)$^{\hspace{0.4em}}$ & 0.993(0.002)$^{\hspace{0.4em}}$ & 0.990(0.003)$^{\hspace{0.4em}}$ & 0.988(0.003)$^{\hspace{0.4em}}$ & 0.993(0.003)$^{\hspace{0.4em}}$ & 0.991(0.003)$^{\hspace{0.4em}}$ \\
359973 & christine & 0.828(0.012)$^{\hspace{0.4em}}$ & 0.831(0.015)$^{\hspace{0.4em}}$ & 0.817(0.012)$^{\hspace{0.4em}}$ & 0.822(0.013)$^{\hspace{0.4em}}$ & 0.829(0.018)$^{\hspace{0.4em}}$ & 0.824(0.011)$^{\hspace{0.4em}}$ & 0.832(0.013)$^{\hspace{0.4em}}$ & 0.825(0.014)$^{\hspace{0.4em}}$ & 0.794(0.048)$^{2}$ \\
359975 & satellite & 0.997(0.004)$^{\hspace{0.4em}}$ & 0.993(0.007)$^{\hspace{0.4em}}$ & 0.995(0.008)$^{\hspace{0.4em}}$ & 0.993(0.007)$^{\hspace{0.4em}}$ & 0.997(0.003)$^{\hspace{0.4em}}$ & 0.994(0.006)$^{\hspace{0.4em}}$ & 0.985(0.026)$^{\hspace{0.4em}}$ & 0.994(0.007)$^{2}$ & 0.997(0.002)$^{\hspace{0.4em}}$ \\
359979 & amazon\_e... & 0.899(0.012)$^{\hspace{0.4em}}$ & 0.853(0.015)$^{\hspace{0.4em}}$ & 0.876(0.012)$^{\hspace{0.4em}}$ & 0.901(0.012)$^{\hspace{0.4em}}$ & 0.863(0.013)$^{\hspace{0.4em}}$ & 0.879(0.010)$^{\hspace{0.4em}}$ & 0.902(0.011)$^{\hspace{0.4em}}$ & 0.905(0.013)$^{\hspace{0.4em}}$ & 0.865(0.012)$^{\hspace{0.4em}}$ \\
359980 & nomao & 0.997(0.001)$^{\hspace{0.4em}}$ & 0.996(0.001)$^{\hspace{0.4em}}$ & 0.996(0.001)$^{\hspace{0.4em}}$ & 0.997(0.001)$^{\hspace{0.4em}}$ & 0.996(0.001)$^{\hspace{0.4em}}$ & 0.996(0.001)$^{\hspace{0.4em}}$ & 0.998(0.001)$^{1}$ & 0.996(0.001)$^{5}$ & 0.993(0.008)$^{\hspace{0.4em}}$ \\
359982 & bank-mar... & 0.941(0.006)$^{\hspace{0.4em}}$ & 0.939(0.006)$^{\hspace{0.4em}}$ & 0.939(0.007)$^{\hspace{0.4em}}$ & 0.938(0.007)$^{\hspace{0.4em}}$ & 0.937(0.006)$^{\hspace{0.4em}}$ & 0.939(0.007)$^{\hspace{0.4em}}$ & 0.940(0.005)$^{1}$ & 0.940(0.004)$^{6}$ & 0.933(0.007)$^{\hspace{0.4em}}$ \\
359983 & adult & 0.932(0.003)$^{\hspace{0.4em}}$ & 0.930(0.004)$^{\hspace{0.4em}}$ & 0.931(0.004)$^{\hspace{0.4em}}$ & 0.931(0.004)$^{\hspace{0.4em}}$ & 0.929(0.004)$^{\hspace{0.4em}}$ & 0.931(0.004)$^{\hspace{0.4em}}$ & 0.933(0.004)$^{\hspace{0.4em}}$ & -$\hspace{0.4em}$ & 0.927(0.005)$^{\hspace{0.4em}}$ \\
359988 & guillermo & 0.925(0.007)$^{\hspace{0.4em}}$ & 0.913(0.008)$^{\hspace{0.4em}}$ & 0.904(0.008)$^{\hspace{0.4em}}$ & 0.921(0.010)$^{6}$ & 0.875(0.026)$^{\hspace{0.4em}}$ & 0.902(0.010)$^{\hspace{0.4em}}$ & 0.939(0.006)$^{\hspace{0.4em}}$ & 0.916(0.009)$^{\hspace{0.4em}}$ & 0.811(0.032)$^{\hspace{0.4em}}$ \\
359989 & riccardo & 1.000(0.000)$^{\hspace{0.4em}}$ & 1.000(0.000)$^{\hspace{0.4em}}$ & 1.000(0.000)$^{\hspace{0.4em}}$ & 0.999(0.002)$^{1}$ & 0.999(0.000)$^{\hspace{0.4em}}$ & 1.000(0.000)$^{\hspace{0.4em}}$ & 1.000(0.000)$^{\hspace{0.4em}}$ & 1.000(0.000)$^{\hspace{0.4em}}$ & 0.998(0.001)$^{\hspace{0.4em}}$ \\
359990 & miniboone & 0.989(0.001)$^{\hspace{0.4em}}$ & 0.987(0.001)$^{\hspace{0.4em}}$ & 0.988(0.001)$^{\hspace{0.4em}}$ & 0.987(0.001)$^{\hspace{0.4em}}$ & 0.982(0.002)$^{\hspace{0.4em}}$ & 0.987(0.001)$^{\hspace{0.4em}}$ & 0.988(0.001)$^{\hspace{0.4em}}$ & 0.987(0.001)$^{\hspace{0.4em}}$ & 0.981(0.002)$^{\hspace{0.4em}}$ \\
359991 & kick & 0.788(0.007)$^{\hspace{0.4em}}$ & 0.786(0.006)$^{\hspace{0.4em}}$ & 0.785(0.006)$^{\hspace{0.4em}}$ & 0.787(0.007)$^{\hspace{0.4em}}$ & 0.786(0.007)$^{\hspace{0.4em}}$ & 0.788(0.007)$^{\hspace{0.4em}}$ & 0.783(0.007)$^{\hspace{0.4em}}$ & 0.752(0.009)$^{\hspace{0.4em}}$ & 0.728(0.012)$^{\hspace{0.4em}}$ \\
359992 & click\_pr... & 0.700(0.010)$^{\hspace{0.4em}}$ & 0.700(0.012)$^{\hspace{0.4em}}$ & 0.705(0.012)$^{\hspace{0.4em}}$ & 0.722(0.009)$^{\hspace{0.4em}}$ & 0.660(0.016)$^{\hspace{0.4em}}$ & 0.702(0.014)$^{\hspace{0.4em}}$ & 0.728(0.010)$^{\hspace{0.4em}}$ & 0.709(0.014)$^{\hspace{0.4em}}$ & 0.716(0.012)$^{\hspace{0.4em}}$ \\
359994 & sf-polic... & 0.698(0.001)$^{\hspace{0.4em}}$ & 0.695(0.006)$^{\hspace{0.4em}}$ & 0.705(0.003)$^{\hspace{0.4em}}$ & 0.712(0.008)$^{\hspace{0.4em}}$ & 0.623(0.009)$^{\hspace{0.4em}}$ & 0.700(0.002)$^{\hspace{0.4em}}$ & 0.688(0.002)$^{\hspace{0.4em}}$ & 0.706(0.009)$^{\hspace{0.4em}}$ & 0.654(0.020)$^{1}$ \\
360113 & porto-se... & 0.641(0.004)$^{\hspace{0.4em}}$ & 0.638(0.005)$^{\hspace{0.4em}}$ & 0.638(0.004)$^{\hspace{0.4em}}$ & 0.642(0.004)$^{\hspace{0.4em}}$ & 0.624(0.007)$^{\hspace{0.4em}}$ & 0.642(0.004)$^{\hspace{0.4em}}$ & 0.641(0.004)$^{\hspace{0.4em}}$ & 0.642(0.004)$^{\hspace{0.4em}}$ & 0.626(0.007)$^{\hspace{0.4em}}$ \\
360114 & higgs & 0.839(0.001)$^{\hspace{0.4em}}$ & 0.832(0.003)$^{\hspace{0.4em}}$ & 0.835(0.002)$^{\hspace{0.4em}}$ & 0.840(0.001)$^{\hspace{0.4em}}$ & 0.786(0.008)$^{\hspace{0.4em}}$ & 0.832(0.001)$^{\hspace{0.4em}}$ & 0.838(0.001)$^{\hspace{0.4em}}$ & 0.836(0.001)$^{\hspace{0.4em}}$ & 0.773(0.003)$^{\hspace{0.4em}}$ \\
360975 & kddcup09... & 0.902(0.007)$^{\hspace{0.4em}}$ & 0.892(0.009)$^{1}$ & 0.893(0.009)$^{\hspace{0.4em}}$ & -$\hspace{0.4em}$ & -$\hspace{0.4em}$ & 0.898(0.008)$^{\hspace{0.4em}}$ & 0.910(0.007)$^{\hspace{0.4em}}$ & 0.907(0.006)$^{\hspace{0.4em}}$ & -$\hspace{0.4em}$ \\
3945 & kddcup09... & 0.846(0.013)$^{\hspace{0.4em}}$ & 0.838(0.015)$^{\hspace{0.4em}}$ & 0.841(0.015)$^{\hspace{0.4em}}$ & 0.829(0.010)$^{\hspace{0.4em}}$ & 0.830(0.014)$^{\hspace{0.4em}}$ & 0.838(0.015)$^{\hspace{0.4em}}$ & 0.851(0.008)$^{6}$ & 0.841(0.016)$^{2}$ & 0.823(0.015)$^{1}$ \\
\bottomrule
\end{tabular}
\caption{Results for binary classification (in AUC) on a one hour budget, denoted as \texttt{mean}(\texttt{std})$^{\mbox{\texttt{fails}}}$.}
\label{tab:auc-1h8c_gp3}
\end{table}
\end{landscape}
