# Supplementary material for: AMLB: an AutoML Benchmark
Source: arXiv:2207.12560 source file (2023-11-16)
Supplement: Supplementary file 3 [file errors-per-subgroup.tex]

\begin{table}
\caption{An overview of errors for framework (A-H). `tasks' denote how many unique tasks are affected, and `total' how frequent the error occurred in total.}
\begin{tabular}{llllrr}
 &  &  &  & Tasks & Total \\
framework & ttype & constraint & error &  &  \\
autogluon & Classification & 4h & Memory & 2 & 3 \\
\multirow{4}{*}{autosklearn} & \multirow{2}{*}{Classification} & 1h & Memory & 1 & 1 \\
 &  & 4h & Timeout & 1 & 5 \\
 & \multirow{2}{*}{Regression} & 1h & Data & 1 & 1 \\
 &  & 4h & Data & 1 & 1 \\
autosklearn2 & Classification & 4h & Timeout & 1 & 10 \\
\multirow{6}{*}{flaml} & \multirow{4}{*}{Classification} & 1h & Memory & 4 & 18 \\
 &  & \multirow{3}{*}{4h} &  & 1 & 1 \\
 &  &  & Memory & 10 & 51 \\
 &  &  & Timeout & 4 & 8 \\
 & \multirow{2}{*}{Regression} & \multirow{2}{*}{4h} & Memory & 6 & 7 \\
 &  &  & Timeout & 1 & 3 \\
\multirow{7}{*}{gama} & \multirow{6}{*}{Classification} & \multirow{3}{*}{1h} & Data & 1 & 2 \\
 &  &  & Implementation & 4 & 26 \\
 &  &  & Memory & 2 & 9 \\
 &  & \multirow{3}{*}{4h} & Data & 1 & 2 \\
 &  &  & Implementation & 4 & 28 \\
 &  &  & Memory & 5 & 25 \\
 & Regression & 4h & Memory & 2 & 7 \\
\multirow{2}{*}{h2oautoml} & \multirow{2}{*}{Classification} & 1h & Timeout & 1 & 10 \\
 &  & 4h & Timeout & 1 & 10 \\
\end{tabular}
\end{table}

\begin{table}
\caption{An overview of errors for framework (I-Z). `tasks' denote how many unique tasks are affected, and `total' how frequent the error occurred in total.}
\begin{tabular}{llllrr}
 &  &  &  & Tasks & Total \\
framework & ttype & constraint & error &  &  \\
\multirow{6}{*}{lightautoml} & \multirow{4}{*}{Classification} & \multirow{2}{*}{1h} & Memory & 8 & 41 \\
 &  &  & Timeout & 2 & 2 \\
 &  & \multirow{2}{*}{4h} & Memory & 10 & 69 \\
 &  &  & Timeout & 2 & 2 \\
 & \multirow{2}{*}{Regression} & 1h & Memory & 1 & 1 \\
 &  & 4h & Memory & 1 & 5 \\
\multirow{9}{*}{mljarsupervised} & \multirow{6}{*}{Classification} & \multirow{3}{*}{1h} &  & 1 & 1 \\
 &  &  & Implementation & 14 & 72 \\
 &  &  & Memory & 1 & 7 \\
 &  & \multirow{3}{*}{4h} & Implementation & 15 & 118 \\
 &  &  & Memory & 2 & 9 \\
 &  &  & Timeout & 3 & 13 \\
 & \multirow{3}{*}{Regression} & 1h & Data & 1 & 8 \\
 &  & \multirow{2}{*}{4h} & Data & 1 & 5 \\
 &  &  & Timeout & 1 & 1 \\
\multirow{2}{*}{mlr3automl} & \multirow{2}{*}{Classification} & 1h & Memory & 2 & 13 \\
 &  & 4h & Memory & 2 & 20 \\
\multirow{10}{*}{tpot} & \multirow{6}{*}{Classification} & \multirow{3}{*}{1h} & Data & 3 & 12 \\
 &  &  & Implementation & 4 & 12 \\
 &  &  & Timeout & 6 & 27 \\
 &  & \multirow{3}{*}{4h} & Data & 3 & 14 \\
 &  &  & Implementation & 5 & 10 \\
 &  &  & Timeout & 9 & 29 \\
 & \multirow{4}{*}{Regression} & \multirow{2}{*}{1h} & Implementation & 3 & 4 \\
 &  &  & Timeout & 1 & 1 \\
 &  & \multirow{2}{*}{4h} & Implementation & 1 & 4 \\
 &  &  & Memory & 1 & 1 \\
\end{tabular}
\end{table}
