# Supplementary material for: AMLB: an AutoML Benchmark
Source: arXiv:2207.12560 source file (2023-11-16)
Supplement: Supplementary file 4 [file neg_logloss-1h8c_gp3-table.tex]

\footnotesize
\begin{landscape}
\begin{table}
\tiny
\begin{tabular}{rlrrrrrrrrr}
\toprule
 & framework& \unsizedsystemcase{autogluon}\ \ \  & \unsizedsystemcase{auto-sklearn}\ \ \  & \unsizedsystemcase{auto-sklearn 2} & \unsizedsystemcase{flaml}\ \ \ & \unsizedsystemcase{gama}\ \ \ & \unsizedsystemcase{h2o automl}\ \ \  & \unsizedsystemcase{light automl}\ \ \  & \unsizedsystemcase{mljar}\ \ \  & \unsizedsystemcase{tpot}\ \ \  \\
 task id & task name & & & & & & & & & \\
\midrule
10090 & amazon-c... & 0.722(0.094)$^{\hspace{0.4em}}$ & 0.852(0.164)$^{\hspace{0.4em}}$ & 0.842(0.143)$^{\hspace{0.4em}}$ & 1.122(0.179)$^{\hspace{0.4em}}$ & 0.900(0.080)$^{\hspace{0.4em}}$ & 1.196(0.209)$^{\hspace{0.4em}}$ & 0.844(0.097)$^{\hspace{0.4em}}$ & 1.211(0.163)$^{\hspace{0.4em}}$ & 1.169(0.294)$^{3}$ \\
168784 & steel-pl... & 0.465(0.041)$^{\hspace{0.4em}}$ & 0.530(0.029)$^{\hspace{0.4em}}$ & 0.472(0.031)$^{\hspace{0.4em}}$ & 0.509(0.047)$^{\hspace{0.4em}}$ & 0.486(0.033)$^{\hspace{0.4em}}$ & 0.484(0.039)$^{\hspace{0.4em}}$ & 0.488(0.027)$^{\hspace{0.4em}}$ & 0.464(0.027)$^{\hspace{0.4em}}$ & 0.511(0.041)$^{\hspace{0.4em}}$ \\
168909 & dilbert & 0.012(0.004)$^{\hspace{0.4em}}$ & 0.033(0.012)$^{\hspace{0.4em}}$ & 0.052(0.020)$^{\hspace{0.4em}}$ & 0.024(0.010)$^{\hspace{0.4em}}$ & 0.169(0.031)$^{\hspace{0.4em}}$ & 0.044(0.007)$^{\hspace{0.4em}}$ & 0.033(0.006)$^{\hspace{0.4em}}$ & 0.028(0.010)$^{\hspace{0.4em}}$ & 0.166(0.103)$^{\hspace{0.4em}}$ \\
168910 & fabert & 0.686(0.027)$^{\hspace{0.4em}}$ & 0.744(0.029)$^{\hspace{0.4em}}$ & 0.745(0.024)$^{\hspace{0.4em}}$ & 0.766(0.025)$^{\hspace{0.4em}}$ & 0.753(0.020)$^{\hspace{0.4em}}$ & 0.729(0.031)$^{\hspace{0.4em}}$ & 0.771(0.031)$^{\hspace{0.4em}}$ & 0.758(0.032)$^{\hspace{0.4em}}$ & 0.857(0.041)$^{\hspace{0.4em}}$ \\
189355 & dionis & 0.273(0.004)$^{\hspace{0.4em}}$ & 1.138(0.273)$^{\hspace{0.4em}}$ & 0.594(0.071)$^{\hspace{0.4em}}$ & 0.374(0.004)$^{1}$ & 1.591(0.348)$^{\hspace{0.4em}}$ & 3.351(0.120)$^{\hspace{0.4em}}$ & -$\hspace{0.4em}$ & 1.198(0.421)$^{8}$ & 17.230(nan)$^{9}$ \\
190146 & vehicle & 0.296(0.052)$^{\hspace{0.4em}}$ & 0.365(0.044)$^{\hspace{0.4em}}$ & 0.342(0.041)$^{\hspace{0.4em}}$ & 0.445(0.041)$^{\hspace{0.4em}}$ & 0.357(0.034)$^{\hspace{0.4em}}$ & 0.328(0.062)$^{\hspace{0.4em}}$ & 0.369(0.061)$^{\hspace{0.4em}}$ & 0.328(0.031)$^{\hspace{0.4em}}$ & 0.377(0.072)$^{\hspace{0.4em}}$ \\
2073 & yeast & 1.012(0.084)$^{\hspace{0.4em}}$ & 1.038(0.079)$^{\hspace{0.4em}}$ & 1.011(0.083)$^{\hspace{0.4em}}$ & 1.012(0.079)$^{\hspace{0.4em}}$ & 1.020(0.080)$^{5}$ & 1.058(0.094)$^{\hspace{0.4em}}$ & 1.039(0.091)$^{5}$ & 1.007(0.088)$^{\hspace{0.4em}}$ & 1.017(0.081)$^{5}$ \\
211979 & jannis & 0.650(0.005)$^{\hspace{0.4em}}$ & 0.665(0.006)$^{\hspace{0.4em}}$ & 0.672(0.007)$^{\hspace{0.4em}}$ & 0.676(0.009)$^{\hspace{0.4em}}$ & 0.726(0.012)$^{\hspace{0.4em}}$ & 0.669(0.006)$^{\hspace{0.4em}}$ & 0.665(0.005)$^{\hspace{0.4em}}$ & 0.663(0.005)$^{\hspace{0.4em}}$ & 0.732(0.011)$^{\hspace{0.4em}}$ \\
211986 & diabetes... & 0.833(0.005)$^{\hspace{0.4em}}$ & 0.835(0.006)$^{\hspace{0.4em}}$ & 0.834(0.006)$^{\hspace{0.4em}}$ & 0.833(0.006)$^{\hspace{0.4em}}$ & 0.844(0.006)$^{\hspace{0.4em}}$ & 0.833(0.006)$^{\hspace{0.4em}}$ & 0.763(0.007)$^{\hspace{0.4em}}$ & 0.829(0.006)$^{\hspace{0.4em}}$ & 0.848(0.007)$^{\hspace{0.4em}}$ \\
359953 & micro-ma... & 0.257(0.084)$^{\hspace{0.4em}}$ & 0.291(0.138)$^{\hspace{0.4em}}$ & 0.210(0.076)$^{\hspace{0.4em}}$ & 0.329(0.109)$^{\hspace{0.4em}}$ & 0.242(0.113)$^{\hspace{0.4em}}$ & 0.387(0.135)$^{\hspace{0.4em}}$ & 0.272(0.072)$^{\hspace{0.4em}}$ & 0.432(0.228)$^{\hspace{0.4em}}$ & 0.375(0.139)$^{\hspace{0.4em}}$ \\
359954 & eucalypt... & 0.690(0.053)$^{\hspace{0.4em}}$ & 0.742(0.075)$^{\hspace{0.4em}}$ & 0.692(0.053)$^{\hspace{0.4em}}$ & 0.728(0.058)$^{\hspace{0.4em}}$ & 0.698(0.053)$^{\hspace{0.4em}}$ & 0.689(0.052)$^{\hspace{0.4em}}$ & 0.703(0.064)$^{\hspace{0.4em}}$ & 0.648(0.047)$^{\hspace{0.4em}}$ & 0.696(0.064)$^{\hspace{0.4em}}$ \\
359957 & cnae-9 & 0.137(0.066)$^{\hspace{0.4em}}$ & 0.176(0.076)$^{\hspace{0.4em}}$ & 0.146(0.049)$^{\hspace{0.4em}}$ & 0.165(0.049)$^{\hspace{0.4em}}$ & 0.125(0.044)$^{\hspace{0.4em}}$ & 0.162(0.081)$^{\hspace{0.4em}}$ & 0.152(0.058)$^{\hspace{0.4em}}$ & 0.207(0.097)$^{\hspace{0.4em}}$ & 0.155(0.067)$^{\hspace{0.4em}}$ \\
359959 & cmc & 0.916(0.055)$^{\hspace{0.4em}}$ & 0.883(0.038)$^{\hspace{0.4em}}$ & 0.882(0.041)$^{\hspace{0.4em}}$ & 0.897(0.040)$^{\hspace{0.4em}}$ & 0.893(0.043)$^{\hspace{0.4em}}$ & 0.902(0.044)$^{\hspace{0.4em}}$ & 0.885(0.046)$^{\hspace{0.4em}}$ & 0.893(0.056)$^{\hspace{0.4em}}$ & 0.918(0.059)$^{\hspace{0.4em}}$ \\
359960 & car & 0.005(0.014)$^{\hspace{0.4em}}$ & 0.003(0.005)$^{\hspace{0.4em}}$ & 0.001(0.002)$^{\hspace{0.4em}}$ & 0.003(0.002)$^{\hspace{0.4em}}$ & 0.015(0.009)$^{\hspace{0.4em}}$ & 0.002(0.003)$^{\hspace{0.4em}}$ & 0.002(0.002)$^{\hspace{0.4em}}$ & 0.063(0.188)$^{\hspace{0.4em}}$ & 0.812(1.332)$^{\hspace{0.4em}}$ \\
359961 & mfeat-fa... & 0.069(0.028)$^{\hspace{0.4em}}$ & 0.092(0.038)$^{\hspace{0.4em}}$ & 0.074(0.031)$^{\hspace{0.4em}}$ & 0.086(0.041)$^{\hspace{0.4em}}$ & 0.078(0.030)$^{\hspace{0.4em}}$ & 0.095(0.054)$^{\hspace{0.4em}}$ & 0.085(0.029)$^{\hspace{0.4em}}$ & 0.101(0.040)$^{\hspace{0.4em}}$ & 0.113(0.066)$^{\hspace{0.4em}}$ \\
359963 & segment & 0.141(0.039)$^{\hspace{0.4em}}$ & 0.178(0.039)$^{\hspace{0.4em}}$ & 0.152(0.031)$^{\hspace{0.4em}}$ & 0.175(0.062)$^{\hspace{0.4em}}$ & 0.149(0.031)$^{\hspace{0.4em}}$ & 0.157(0.040)$^{\hspace{0.4em}}$ & 0.161(0.036)$^{\hspace{0.4em}}$ & 0.156(0.036)$^{\hspace{0.4em}}$ & 0.164(0.038)$^{\hspace{0.4em}}$ \\
359964 & dna & 0.106(0.028)$^{\hspace{0.4em}}$ & 0.119(0.032)$^{\hspace{0.4em}}$ & 0.111(0.026)$^{\hspace{0.4em}}$ & 0.111(0.030)$^{\hspace{0.4em}}$ & 0.106(0.028)$^{\hspace{0.4em}}$ & 0.111(0.029)$^{\hspace{0.4em}}$ & 0.109(0.025)$^{\hspace{0.4em}}$ & 0.113(0.027)$^{\hspace{0.4em}}$ & 0.117(0.028)$^{\hspace{0.4em}}$ \\
359969 & first-or... & 1.037(0.041)$^{\hspace{0.4em}}$ & 1.104(0.032)$^{\hspace{0.4em}}$ & 1.047(0.032)$^{\hspace{0.4em}}$ & 1.040(0.031)$^{\hspace{0.4em}}$ & 1.057(0.029)$^{\hspace{0.4em}}$ & 1.042(0.033)$^{\hspace{0.4em}}$ & 1.048(0.024)$^{\hspace{0.4em}}$ & 1.035(0.028)$^{\hspace{0.4em}}$ & 1.072(0.021)$^{\hspace{0.4em}}$ \\
359970 & gesturep... & 0.653(0.032)$^{\hspace{0.4em}}$ & 0.803(0.026)$^{\hspace{0.4em}}$ & 0.774(0.039)$^{\hspace{0.4em}}$ & 0.773(0.036)$^{\hspace{0.4em}}$ & 0.818(0.031)$^{\hspace{0.4em}}$ & 0.717(0.039)$^{\hspace{0.4em}}$ & 0.755(0.038)$^{\hspace{0.4em}}$ & 0.722(0.034)$^{\hspace{0.4em}}$ & 0.860(0.055)$^{\hspace{0.4em}}$ \\
359974 & wine-qua... & 0.700(0.027)$^{\hspace{0.4em}}$ & 0.797(0.041)$^{\hspace{0.4em}}$ & 0.723(0.032)$^{\hspace{0.4em}}$ & 0.732(0.042)$^{\hspace{0.4em}}$ & 0.755(0.020)$^{5}$ & 0.751(0.029)$^{\hspace{0.4em}}$ & 0.813(0.013)$^{5}$ & 0.772(0.033)$^{\hspace{0.4em}}$ & 0.808(0.025)$^{5}$ \\
359976 & fashion-... & 0.237(0.007)$^{\hspace{0.4em}}$ & 0.253(0.008)$^{\hspace{0.4em}}$ & 0.263(0.010)$^{\hspace{0.4em}}$ & 0.259(0.021)$^{\hspace{0.4em}}$ & 0.400(0.017)$^{\hspace{0.4em}}$ & 0.278(0.008)$^{\hspace{0.4em}}$ & 0.250(0.008)$^{\hspace{0.4em}}$ & 0.249(0.009)$^{\hspace{0.4em}}$ & 0.515(0.113)$^{\hspace{0.4em}}$ \\
359977 & connect-4 & 0.294(0.007)$^{\hspace{0.4em}}$ & 0.355(0.013)$^{\hspace{0.4em}}$ & 0.351(0.027)$^{\hspace{0.4em}}$ & 0.347(0.007)$^{\hspace{0.4em}}$ & 0.384(0.031)$^{\hspace{0.4em}}$ & 0.309(0.007)$^{\hspace{0.4em}}$ & 0.337(0.007)$^{\hspace{0.4em}}$ & 0.323(0.006)$^{\hspace{0.4em}}$ & 0.399(0.040)$^{\hspace{0.4em}}$ \\
359981 & jungle\_c... & 0.011(0.002)$^{\hspace{0.4em}}$ & 0.186(0.036)$^{\hspace{0.4em}}$ & 0.233(0.022)$^{\hspace{0.4em}}$ & 0.210(0.006)$^{\hspace{0.4em}}$ & 0.240(0.015)$^{\hspace{0.4em}}$ & 0.171(0.025)$^{\hspace{0.4em}}$ & 0.148(0.018)$^{\hspace{0.4em}}$ & 0.082(0.011)$^{\hspace{0.4em}}$ & 0.552(1.073)$^{\hspace{0.4em}}$ \\
359984 & helena & 2.464(0.014)$^{\hspace{0.4em}}$ & 2.554(0.019)$^{\hspace{0.4em}}$ & 2.493(0.019)$^{\hspace{0.4em}}$ & 2.584(0.022)$^{\hspace{0.4em}}$ & 2.786(0.011)$^{7}$ & 2.781(0.020)$^{\hspace{0.4em}}$ & 2.554(0.017)$^{\hspace{0.4em}}$ & 2.601(0.032)$^{\hspace{0.4em}}$ & 2.981(0.095)$^{\hspace{0.4em}}$ \\
359985 & volkert & 0.691(0.015)$^{\hspace{0.4em}}$ & 0.790(0.016)$^{\hspace{0.4em}}$ & 0.817(0.019)$^{\hspace{0.4em}}$ & 0.834(0.074)$^{\hspace{0.4em}}$ & 1.025(0.016)$^{\hspace{0.4em}}$ & 0.833(0.014)$^{\hspace{0.4em}}$ & 0.832(0.013)$^{\hspace{0.4em}}$ & 0.793(0.015)$^{\hspace{0.4em}}$ & 1.006(0.023)$^{\hspace{0.4em}}$ \\
359986 & robert & 1.444(0.014)$^{\hspace{0.4em}}$ & 1.404(0.042)$^{\hspace{0.4em}}$ & 1.476(0.048)$^{\hspace{0.4em}}$ & 1.377(0.028)$^{\hspace{0.4em}}$ & 1.697(0.058)$^{\hspace{0.4em}}$ & 1.507(0.064)$^{\hspace{0.4em}}$ & 1.317(0.021)$^{\hspace{0.4em}}$ & 1.342(0.035)$^{\hspace{0.4em}}$ & 2.017(0.161)$^{\hspace{0.4em}}$ \\
359987 & shuttle & 0.000(0.000)$^{\hspace{0.4em}}$ & 0.000(0.000)$^{\hspace{0.4em}}$ & 0.000(0.000)$^{\hspace{0.4em}}$ & 0.000(0.001)$^{\hspace{0.4em}}$ & 0.001(0.000)$^{\hspace{0.4em}}$ & 0.000(0.001)$^{\hspace{0.4em}}$ & 0.001(0.000)$^{\hspace{0.4em}}$ & 0.000(0.000)$^{\hspace{0.4em}}$ & 0.001(0.000)$^{\hspace{0.4em}}$ \\
359993 & okcupid-... & 0.559(0.009)$^{\hspace{0.4em}}$ & 0.568(0.006)$^{\hspace{0.4em}}$ & 0.567(0.008)$^{\hspace{0.4em}}$ & 0.565(0.008)$^{\hspace{0.4em}}$ & 0.568(0.007)$^{\hspace{0.4em}}$ & 0.565(0.011)$^{\hspace{0.4em}}$ & 0.560(0.009)$^{\hspace{0.4em}}$ & 0.564(0.008)$^{\hspace{0.4em}}$ & 0.572(0.008)$^{\hspace{0.4em}}$ \\
360112 & kddcup99 & 0.002(0.000)$^{\hspace{0.4em}}$ & 0.001(0.002)$^{\hspace{0.4em}}$ & 0.000(0.000)$^{\hspace{0.4em}}$ & 0.000(0.000)$^{\hspace{0.4em}}$ & -$\hspace{0.4em}$ & -$\hspace{0.4em}$ & -$\hspace{0.4em}$ & 0.000(0.000)$^{\hspace{0.4em}}$ & -$\hspace{0.4em}$ \\
7593 & covertype & 0.065(0.001)$^{\hspace{0.4em}}$ & 0.141(0.013)$^{\hspace{0.4em}}$ & 0.113(0.005)$^{\hspace{0.4em}}$ & 0.068(0.002)$^{\hspace{0.4em}}$ & 0.529(0.039)$^{\hspace{0.4em}}$ & 0.111(0.003)$^{\hspace{0.4em}}$ & 0.085(0.001)$^{\hspace{0.4em}}$ & 0.084(0.008)$^{\hspace{0.4em}}$ & 0.537(0.095)$^{\hspace{0.4em}}$ \\
\bottomrule
\end{tabular}
\caption{Results for multiclass classification (in logloss) on a one hour budget, denoted as \texttt{mean}(\texttt{std})$^{\mbox{\texttt{fails}}}$.}
\label{tab:neg_logloss-1h8c_gp3}
\end{table}
\end{landscape}
