# Supplementary material for: AMLB: an AutoML Benchmark
Source: arXiv:2207.12560 source file (2023-11-16)
Supplement: Supplementary file 5 [file neg_logloss-4h8c_gp3-table.tex]

\footnotesize
\begin{landscape}
\begin{table}
\tiny
\begin{tabular}{rlrrrrrrrrr}
\toprule
 & framework& \unsizedsystemcase{autogluon}\ \ \  & \unsizedsystemcase{auto-sklearn}\ \ \  & \unsizedsystemcase{auto-sklearn 2} & \unsizedsystemcase{flaml}\ \ \ & \unsizedsystemcase{gama}\ \ \ & \unsizedsystemcase{h2o automl}\ \ \  & \unsizedsystemcase{light automl}\ \ \  & \unsizedsystemcase{mljar}\ \ \  & \unsizedsystemcase{tpot}\ \ \  \\
 task id & task name & & & & & & & & & \\
\midrule
10090 & amazon-c... & 0.635(0.058)$^{\hspace{0.4em}}$ & 0.809(0.122)$^{\hspace{0.4em}}$ & 0.837(0.122)$^{\hspace{0.4em}}$ & 1.144(0.163)$^{\hspace{0.4em}}$ & 0.907(0.094)$^{\hspace{0.4em}}$ & 1.172(0.167)$^{\hspace{0.4em}}$ & 0.808(0.062)$^{\hspace{0.4em}}$ & 1.181(0.132)$^{\hspace{0.4em}}$ & 0.852(0.159)$^{2}$ \\
168784 & steel-pl... & 0.466(0.041)$^{\hspace{0.4em}}$ & 0.512(0.028)$^{\hspace{0.4em}}$ & 0.472(0.029)$^{\hspace{0.4em}}$ & 0.505(0.052)$^{\hspace{0.4em}}$ & 0.491(0.039)$^{\hspace{0.4em}}$ & 0.490(0.042)$^{\hspace{0.4em}}$ & 0.488(0.033)$^{\hspace{0.4em}}$ & 0.467(0.032)$^{\hspace{0.4em}}$ & 0.486(0.021)$^{\hspace{0.4em}}$ \\
168909 & dilbert & 0.012(0.004)$^{\hspace{0.4em}}$ & 0.033(0.012)$^{\hspace{0.4em}}$ & 0.029(0.008)$^{\hspace{0.4em}}$ & 0.026(0.009)$^{\hspace{0.4em}}$ & 0.115(0.044)$^{\hspace{0.4em}}$ & 0.023(0.005)$^{\hspace{0.4em}}$ & 0.032(0.006)$^{\hspace{0.4em}}$ & 0.024(0.009)$^{\hspace{0.4em}}$ & 0.060(0.022)$^{\hspace{0.4em}}$ \\
168910 & fabert & 0.682(0.028)$^{\hspace{0.4em}}$ & 0.756(0.035)$^{\hspace{0.4em}}$ & 0.733(0.026)$^{\hspace{0.4em}}$ & 0.762(0.025)$^{\hspace{0.4em}}$ & 0.737(0.029)$^{\hspace{0.4em}}$ & 0.728(0.031)$^{\hspace{0.4em}}$ & 0.781(0.034)$^{\hspace{0.4em}}$ & 0.752(0.025)$^{\hspace{0.4em}}$ & 0.795(0.049)$^{\hspace{0.4em}}$ \\
189355 & dionis & 0.248(0.004)$^{\hspace{0.4em}}$ & 0.491(0.037)$^{\hspace{0.4em}}$ & 0.523(0.144)$^{\hspace{0.4em}}$ & -$\hspace{0.4em}$ & 1.587(0.244)$^{\hspace{0.4em}}$ & 1.469(0.127)$^{\hspace{0.4em}}$ & -$\hspace{0.4em}$ & -$\hspace{0.4em}$ & -$\hspace{0.4em}$ \\
190146 & vehicle & 0.298(0.050)$^{\hspace{0.4em}}$ & 0.368(0.055)$^{\hspace{0.4em}}$ & 0.329(0.030)$^{\hspace{0.4em}}$ & 0.442(0.049)$^{\hspace{0.4em}}$ & 0.369(0.032)$^{\hspace{0.4em}}$ & 0.331(0.062)$^{\hspace{0.4em}}$ & 0.397(0.066)$^{\hspace{0.4em}}$ & 0.321(0.043)$^{\hspace{0.4em}}$ & 0.339(0.065)$^{\hspace{0.4em}}$ \\
2073 & yeast & 1.015(0.087)$^{\hspace{0.4em}}$ & 1.043(0.080)$^{\hspace{0.4em}}$ & 1.015(0.084)$^{\hspace{0.4em}}$ & 1.011(0.083)$^{\hspace{0.4em}}$ & 1.019(0.081)$^{5}$ & 1.040(0.091)$^{\hspace{0.4em}}$ & 1.038(0.094)$^{5}$ & 1.004(0.085)$^{\hspace{0.4em}}$ & 1.029(0.083)$^{5}$ \\
211979 & jannis & 0.647(0.006)$^{\hspace{0.4em}}$ & 0.666(0.010)$^{\hspace{0.4em}}$ & 0.672(0.005)$^{\hspace{0.4em}}$ & 0.675(0.011)$^{\hspace{0.4em}}$ & 0.698(0.009)$^{\hspace{0.4em}}$ & 0.665(0.006)$^{\hspace{0.4em}}$ & 0.665(0.005)$^{\hspace{0.4em}}$ & 0.658(0.005)$^{\hspace{0.4em}}$ & 0.715(0.011)$^{\hspace{0.4em}}$ \\
211986 & diabetes... & 0.831(0.006)$^{\hspace{0.4em}}$ & 0.834(0.005)$^{\hspace{0.4em}}$ & 0.832(0.005)$^{\hspace{0.4em}}$ & 0.832(0.006)$^{\hspace{0.4em}}$ & 0.837(0.006)$^{\hspace{0.4em}}$ & 0.833(0.006)$^{\hspace{0.4em}}$ & 0.762(0.008)$^{\hspace{0.4em}}$ & 0.828(0.006)$^{\hspace{0.4em}}$ & 0.843(0.005)$^{\hspace{0.4em}}$ \\
359953 & micro-ma... & 0.252(0.088)$^{\hspace{0.4em}}$ & 0.271(0.093)$^{\hspace{0.4em}}$ & 0.189(0.073)$^{\hspace{0.4em}}$ & 0.307(0.129)$^{\hspace{0.4em}}$ & 0.223(0.092)$^{\hspace{0.4em}}$ & 0.329(0.152)$^{\hspace{0.4em}}$ & 0.284(0.112)$^{\hspace{0.4em}}$ & 0.460(0.202)$^{\hspace{0.4em}}$ & 0.289(0.153)$^{\hspace{0.4em}}$ \\
359954 & eucalypt... & 0.690(0.053)$^{\hspace{0.4em}}$ & 0.716(0.047)$^{\hspace{0.4em}}$ & 0.704(0.061)$^{\hspace{0.4em}}$ & 0.779(0.121)$^{\hspace{0.4em}}$ & 0.700(0.057)$^{\hspace{0.4em}}$ & 0.702(0.087)$^{\hspace{0.4em}}$ & 0.695(0.058)$^{\hspace{0.4em}}$ & 0.646(0.054)$^{\hspace{0.4em}}$ & 0.752(0.130)$^{\hspace{0.4em}}$ \\
359957 & cnae-9 & 0.137(0.068)$^{\hspace{0.4em}}$ & 0.178(0.076)$^{\hspace{0.4em}}$ & 0.143(0.043)$^{\hspace{0.4em}}$ & 0.139(0.048)$^{\hspace{0.4em}}$ & 0.132(0.044)$^{\hspace{0.4em}}$ & 0.164(0.103)$^{\hspace{0.4em}}$ & 0.149(0.058)$^{\hspace{0.4em}}$ & 0.176(0.057)$^{\hspace{0.4em}}$ & 0.150(0.077)$^{\hspace{0.4em}}$ \\
359959 & cmc & 0.920(0.057)$^{\hspace{0.4em}}$ & 0.889(0.043)$^{\hspace{0.4em}}$ & 0.884(0.037)$^{\hspace{0.4em}}$ & 0.899(0.045)$^{\hspace{0.4em}}$ & 0.893(0.043)$^{\hspace{0.4em}}$ & 0.898(0.043)$^{\hspace{0.4em}}$ & 0.887(0.044)$^{\hspace{0.4em}}$ & 0.888(0.054)$^{\hspace{0.4em}}$ & 0.908(0.060)$^{\hspace{0.4em}}$ \\
359960 & car & 0.004(0.011)$^{\hspace{0.4em}}$ & 0.004(0.008)$^{\hspace{0.4em}}$ & 0.002(0.004)$^{\hspace{0.4em}}$ & 0.003(0.005)$^{\hspace{0.4em}}$ & 0.012(0.008)$^{\hspace{0.4em}}$ & 0.001(0.001)$^{\hspace{0.4em}}$ & 0.002(0.002)$^{\hspace{0.4em}}$ & 0.002(0.003)$^{\hspace{0.4em}}$ & 1.450(3.004)$^{\hspace{0.4em}}$ \\
359961 & mfeat-fa... & 0.067(0.028)$^{\hspace{0.4em}}$ & 0.093(0.033)$^{\hspace{0.4em}}$ & 0.074(0.030)$^{\hspace{0.4em}}$ & 0.093(0.042)$^{\hspace{0.4em}}$ & 0.082(0.028)$^{\hspace{0.4em}}$ & 0.098(0.042)$^{\hspace{0.4em}}$ & 0.080(0.029)$^{\hspace{0.4em}}$ & 0.102(0.029)$^{\hspace{0.4em}}$ & 0.108(0.042)$^{\hspace{0.4em}}$ \\
359963 & segment & 0.054(0.024)$^{\hspace{0.4em}}$ & 0.084(0.031)$^{\hspace{0.4em}}$ & 0.062(0.026)$^{\hspace{0.4em}}$ & 0.079(0.041)$^{\hspace{0.4em}}$ & 0.067(0.026)$^{\hspace{0.4em}}$ & 0.159(0.040)$^{\hspace{0.4em}}$ & 0.061(0.021)$^{\hspace{0.4em}}$ & 0.058(0.021)$^{\hspace{0.4em}}$ & 0.071(0.032)$^{\hspace{0.4em}}$ \\
359964 & dna & 0.106(0.027)$^{\hspace{0.4em}}$ & 0.116(0.032)$^{\hspace{0.4em}}$ & 0.111(0.025)$^{\hspace{0.4em}}$ & 0.106(0.029)$^{\hspace{0.4em}}$ & 0.106(0.028)$^{\hspace{0.4em}}$ & 0.109(0.030)$^{\hspace{0.4em}}$ & 0.109(0.026)$^{\hspace{0.4em}}$ & 0.109(0.025)$^{\hspace{0.4em}}$ & 0.112(0.025)$^{\hspace{0.4em}}$ \\
359969 & first-or... & 1.039(0.038)$^{\hspace{0.4em}}$ & 1.103(0.035)$^{\hspace{0.4em}}$ & 1.041(0.030)$^{\hspace{0.4em}}$ & 1.037(0.027)$^{\hspace{0.4em}}$ & 1.052(0.027)$^{\hspace{0.4em}}$ & 1.049(0.039)$^{\hspace{0.4em}}$ & 1.046(0.026)$^{\hspace{0.4em}}$ & 1.032(0.029)$^{\hspace{0.4em}}$ & 1.062(0.035)$^{\hspace{0.4em}}$ \\
359970 & gesturep... & 0.652(0.033)$^{\hspace{0.4em}}$ & 0.807(0.021)$^{\hspace{0.4em}}$ & 0.768(0.029)$^{\hspace{0.4em}}$ & 0.763(0.028)$^{\hspace{0.4em}}$ & 0.807(0.039)$^{\hspace{0.4em}}$ & 0.762(0.032)$^{\hspace{0.4em}}$ & 0.757(0.039)$^{\hspace{0.4em}}$ & 0.720(0.035)$^{\hspace{0.4em}}$ & 0.834(0.044)$^{\hspace{0.4em}}$ \\
359974 & wine-qua... & 0.698(0.027)$^{\hspace{0.4em}}$ & 0.793(0.038)$^{\hspace{0.4em}}$ & 0.715(0.028)$^{\hspace{0.4em}}$ & 0.726(0.050)$^{\hspace{0.4em}}$ & 0.772(0.018)$^{5}$ & 0.757(0.033)$^{\hspace{0.4em}}$ & 0.791(0.021)$^{5}$ & 0.755(0.030)$^{\hspace{0.4em}}$ & 0.787(0.021)$^{5}$ \\
359976 & fashion-... & 0.217(0.009)$^{\hspace{0.4em}}$ & 0.242(0.009)$^{\hspace{0.4em}}$ & 0.247(0.012)$^{\hspace{0.4em}}$ & 0.257(0.032)$^{2}$ & 0.356(0.009)$^{\hspace{0.4em}}$ & 0.253(0.009)$^{\hspace{0.4em}}$ & 0.250(0.008)$^{\hspace{0.4em}}$ & 0.245(0.008)$^{\hspace{0.4em}}$ & 0.415(0.029)$^{\hspace{0.4em}}$ \\
359977 & connect-4 & 0.293(0.007)$^{\hspace{0.4em}}$ & 0.348(0.008)$^{\hspace{0.4em}}$ & 0.342(0.013)$^{\hspace{0.4em}}$ & 0.339(0.005)$^{\hspace{0.4em}}$ & 0.346(0.028)$^{\hspace{0.4em}}$ & 0.318(0.028)$^{\hspace{0.4em}}$ & 0.321(0.006)$^{\hspace{0.4em}}$ & 0.316(0.007)$^{\hspace{0.4em}}$ & 0.378(0.023)$^{\hspace{0.4em}}$ \\
359981 & jungle\_c... & 0.006(0.002)$^{\hspace{0.4em}}$ & 0.171(0.045)$^{\hspace{0.4em}}$ & 0.203(0.021)$^{\hspace{0.4em}}$ & 0.211(0.005)$^{\hspace{0.4em}}$ & 0.217(0.022)$^{\hspace{0.4em}}$ & 0.107(0.011)$^{\hspace{0.4em}}$ & 0.102(0.009)$^{\hspace{0.4em}}$ & 0.073(0.006)$^{\hspace{0.4em}}$ & 1.078(2.885)$^{\hspace{0.4em}}$ \\
359984 & helena & 2.470(0.016)$^{\hspace{0.4em}}$ & 2.526(0.018)$^{\hspace{0.4em}}$ & 2.485(0.031)$^{\hspace{0.4em}}$ & 2.564(0.019)$^{\hspace{0.4em}}$ & 2.731(nan)$^{9}$ & 2.794(0.018)$^{\hspace{0.4em}}$ & 2.504(0.014)$^{\hspace{0.4em}}$ & 2.575(0.021)$^{1}$ & 2.922(0.039)$^{\hspace{0.4em}}$ \\
359985 & volkert & 0.674(0.009)$^{\hspace{0.4em}}$ & 0.780(0.022)$^{\hspace{0.4em}}$ & 0.833(0.038)$^{\hspace{0.4em}}$ & 0.812(0.011)$^{\hspace{0.4em}}$ & 0.951(0.016)$^{\hspace{0.4em}}$ & 0.781(0.012)$^{\hspace{0.4em}}$ & 0.781(0.011)$^{\hspace{0.4em}}$ & 0.794(0.013)$^{\hspace{0.4em}}$ & 0.973(0.040)$^{1}$ \\
359986 & robert & 1.265(0.030)$^{\hspace{0.4em}}$ & 1.324(0.027)$^{\hspace{0.4em}}$ & 1.383(0.031)$^{\hspace{0.4em}}$ & 1.307(0.012)$^{1}$ & 1.617(0.030)$^{\hspace{0.4em}}$ & 1.385(0.025)$^{\hspace{0.4em}}$ & 1.276(0.024)$^{\hspace{0.4em}}$ & 1.306(0.029)$^{\hspace{0.4em}}$ & 1.809(0.114)$^{\hspace{0.4em}}$ \\
359987 & shuttle & 0.000(0.000)$^{\hspace{0.4em}}$ & 0.000(0.001)$^{\hspace{0.4em}}$ & 0.000(0.000)$^{\hspace{0.4em}}$ & 0.000(0.000)$^{\hspace{0.4em}}$ & 0.000(0.000)$^{\hspace{0.4em}}$ & 0.000(0.001)$^{\hspace{0.4em}}$ & 0.001(0.000)$^{\hspace{0.4em}}$ & 0.000(0.000)$^{\hspace{0.4em}}$ & 0.000(0.000)$^{\hspace{0.4em}}$ \\
359993 & okcupid-... & 0.559(0.009)$^{\hspace{0.4em}}$ & 0.567(0.007)$^{\hspace{0.4em}}$ & 0.563(0.008)$^{\hspace{0.4em}}$ & 0.562(0.008)$^{\hspace{0.4em}}$ & 0.568(0.007)$^{\hspace{0.4em}}$ & 0.567(0.008)$^{\hspace{0.4em}}$ & 0.560(0.009)$^{\hspace{0.4em}}$ & 0.563(0.008)$^{\hspace{0.4em}}$ & 0.569(0.009)$^{\hspace{0.4em}}$ \\
360112 & kddcup99 & 0.002(0.000)$^{1}$ & 0.000(0.000)$^{\hspace{0.4em}}$ & 0.000(0.000)$^{\hspace{0.4em}}$ & 0.000(0.000)$^{4}$ & -$\hspace{0.4em}$ & -$\hspace{0.4em}$ & -$\hspace{0.4em}$ & 0.000(0.000)$^{\hspace{0.4em}}$ & -$\hspace{0.4em}$ \\
7593 & covertype & 0.057(0.001)$^{\hspace{0.4em}}$ & 0.097(0.022)$^{\hspace{0.4em}}$ & 0.095(0.010)$^{\hspace{0.4em}}$ & 0.067(0.003)$^{2}$ & 0.255(0.048)$^{4}$ & 0.086(0.002)$^{\hspace{0.4em}}$ & 0.071(0.002)$^{\hspace{0.4em}}$ & 0.083(0.006)$^{\hspace{0.4em}}$ & 0.459(0.139)$^{\hspace{0.4em}}$ \\
\bottomrule
\end{tabular}
\caption{Results for multiclass classification (in logloss) on a four hour budget, denoted as \texttt{mean}(\texttt{std})$^{\mbox{\texttt{fails}}}$.}
\label{tab:neg_logloss-4h8c_gp3}
\end{table}
\end{landscape}
