# Supplementary material for: AMLB: an AutoML Benchmark
Source: arXiv:2207.12560 source file (2023-11-16)
Supplement: Supplementary file 6 [file neg_rmse-1h8c_gp3-table.tex]

\footnotesize
\begin{landscape}
\begin{table}
\tiny
\begin{tabular}{rlrrrrrrrr}
\toprule
 & framework& \unsizedsystemcase{autogluon}\ \ \  & \unsizedsystemcase{auto-sklearn}\ \ \ & \unsizedsystemcase{flaml}\ \ \ & \unsizedsystemcase{gama}\ \ \ & \unsizedsystemcase{h2o automl}\ \ \  & \unsizedsystemcase{light automl}\ \ \  & \unsizedsystemcase{mljar}\ \ \  & \unsizedsystemcase{tpot}\ \ \  \\
 task id & task name & & & & & & & & \\
\midrule
167210 & moneyball & 21(0.85)$^{\hspace{0.4em}}$ & 21(0.61)$^{\hspace{0.4em}}$ & 22(0.83)$^{\hspace{0.4em}}$ & 21(0.79)$^{\hspace{0.4em}}$ & 22(2.2)$^{\hspace{0.4em}}$ & 21(0.71)$^{\hspace{0.4em}}$ & 21(0.84)$^{\hspace{0.4em}}$ & 21(0.85)$^{\hspace{0.4em}}$ \\
233211 & diamonds & 5.1e+02(20)$^{\hspace{0.4em}}$ & 5.2e+02(20)$^{\hspace{0.4em}}$ & 5.2e+02(19)$^{\hspace{0.4em}}$ & 5.2e+02(22)$^{\hspace{0.4em}}$ & 5.1e+02(18)$^{\hspace{0.4em}}$ & 5.2e+02(22)$^{\hspace{0.4em}}$ & 5.1e+02(22)$^{\hspace{0.4em}}$ & 5.4e+02(13)$^{\hspace{0.4em}}$ \\
233212 & allstate... & 1.9e+03(41)$^{\hspace{0.4em}}$ & 1.9e+03(60)$^{\hspace{0.4em}}$ & 1.9e+03(51)$^{\hspace{0.4em}}$ & 2e+03(72)$^{\hspace{0.4em}}$ & 1.9e+03(47)$^{\hspace{0.4em}}$ & 1.9e+03(51)$^{\hspace{0.4em}}$ & 1.9e+03(56)$^{\hspace{0.4em}}$ & 2e+03(62)$^{\hspace{0.4em}}$ \\
233213 & buzzinso... & 1.5e+02(50)$^{\hspace{0.4em}}$ & 1.6e+02(46)$^{\hspace{0.4em}}$ & 1.5e+02(50)$^{\hspace{0.4em}}$ & 1.5e+02(38)$^{\hspace{0.4em}}$ & 1.5e+02(46)$^{\hspace{0.4em}}$ & 1.6e+02(45)$^{\hspace{0.4em}}$ & 1.5e+02(51)$^{\hspace{0.4em}}$ & 1.6e+02(51)$^{1}$ \\
233214 & santande... & 6.8e+06(4.4e+05)$^{\hspace{0.4em}}$ & 6.9e+06(4.4e+05)$^{\hspace{0.4em}}$ & 7e+06(4.4e+05)$^{\hspace{0.4em}}$ & 7e+06(4.9e+05)$^{\hspace{0.4em}}$ & 6.9e+06(4.5e+05)$^{\hspace{0.4em}}$ & 6.9e+06(4.8e+05)$^{1}$ & 6.9e+06(4.7e+05)$^{\hspace{0.4em}}$ & 7e+06(5.1e+05)$^{\hspace{0.4em}}$ \\
233215 & mercedes... & 8.6(1)$^{\hspace{0.4em}}$ & 8.3(1.1)$^{\hspace{0.4em}}$ & 8.3(1.1)$^{\hspace{0.4em}}$ & 8.3(1.1)$^{\hspace{0.4em}}$ & 8.3(1.1)$^{\hspace{0.4em}}$ & 8.3(1.1)$^{\hspace{0.4em}}$ & 8.3(1.1)$^{\hspace{0.4em}}$ & 8.3(1.1)$^{\hspace{0.4em}}$ \\
317614 & yolanda & 8.5(0.041)$^{\hspace{0.4em}}$ & 8.7(0.063)$^{\hspace{0.4em}}$ & 8.6(0.051)$^{\hspace{0.4em}}$ & 9.4(0.066)$^{\hspace{0.4em}}$ & 8.8(0.041)$^{\hspace{0.4em}}$ & 8.6(0.038)$^{\hspace{0.4em}}$ & 8.6(0.064)$^{\hspace{0.4em}}$ & 9.5(0.055)$^{1}$ \\
359929 & airlines... & 29(0.23)$^{\hspace{0.4em}}$ & 29(0.22)$^{\hspace{0.4em}}$ & 29(0.26)$^{\hspace{0.4em}}$ & 29(0.24)$^{\hspace{0.4em}}$ & 29(0.24)$^{\hspace{0.4em}}$ & 29(0.23)$^{\hspace{0.4em}}$ & 29(0.2)$^{\hspace{0.4em}}$ & 29(0.24)$^{3}$ \\
359930 & quake & 0.19(0.0089)$^{\hspace{0.4em}}$ & 0.19(0.0088)$^{\hspace{0.4em}}$ & 0.19(0.0093)$^{\hspace{0.4em}}$ & 0.19(0.0092)$^{\hspace{0.4em}}$ & 0.19(0.01)$^{\hspace{0.4em}}$ & 0.19(0.0098)$^{\hspace{0.4em}}$ & 0.19(0.009)$^{\hspace{0.4em}}$ & 0.19(0.0092)$^{\hspace{0.4em}}$ \\
359931 & sensory & 0.67(0.061)$^{\hspace{0.4em}}$ & 0.7(0.063)$^{\hspace{0.4em}}$ & 0.69(0.052)$^{\hspace{0.4em}}$ & 0.68(0.057)$^{\hspace{0.4em}}$ & 0.69(0.063)$^{\hspace{0.4em}}$ & 0.68(0.062)$^{\hspace{0.4em}}$ & 0.68(0.047)$^{\hspace{0.4em}}$ & 0.69(0.067)$^{\hspace{0.4em}}$ \\
359932 & socmob & 12(7.9)$^{\hspace{0.4em}}$ & 12(4.9)$^{\hspace{0.4em}}$ & 15(8)$^{\hspace{0.4em}}$ & 15(7.5)$^{\hspace{0.4em}}$ & 13(9.6)$^{\hspace{0.4em}}$ & 19(9.1)$^{\hspace{0.4em}}$ & 28(55)$^{\hspace{0.4em}}$ & 17(8.7)$^{\hspace{0.4em}}$ \\
359933 & space\_ga & 0.094(0.013)$^{\hspace{0.4em}}$ & 0.1(0.02)$^{\hspace{0.4em}}$ & 0.1(0.016)$^{\hspace{0.4em}}$ & 0.096(0.019)$^{\hspace{0.4em}}$ & 0.098(0.015)$^{\hspace{0.4em}}$ & 0.1(0.017)$^{\hspace{0.4em}}$ & 0.098(0.018)$^{\hspace{0.4em}}$ & 0.1(0.019)$^{\hspace{0.4em}}$ \\
359934 & tecator & 0.83(0.18)$^{\hspace{0.4em}}$ & 0.67(0.16)$^{\hspace{0.4em}}$ & 0.85(0.16)$^{\hspace{0.4em}}$ & 0.81(0.36)$^{\hspace{0.4em}}$ & 0.65(0.13)$^{\hspace{0.4em}}$ & 0.78(0.25)$^{\hspace{0.4em}}$ & 0.87(0.31)$^{\hspace{0.4em}}$ & 0.62(0.23)$^{\hspace{0.4em}}$ \\
359935 & wine\_qua... & 0.57(0.022)$^{\hspace{0.4em}}$ & 0.6(0.019)$^{\hspace{0.4em}}$ & 0.57(0.021)$^{\hspace{0.4em}}$ & 0.57(0.02)$^{\hspace{0.4em}}$ & 0.58(0.024)$^{\hspace{0.4em}}$ & 0.58(0.023)$^{\hspace{0.4em}}$ & 0.57(0.023)$^{\hspace{0.4em}}$ & 0.58(0.024)$^{\hspace{0.4em}}$ \\
359936 & elevators & 0.0018(5.2e-05)$^{\hspace{0.4em}}$ & 0.002(7.6e-05)$^{\hspace{0.4em}}$ & 0.002(6.6e-05)$^{\hspace{0.4em}}$ & 0.002(6.7e-05)$^{\hspace{0.4em}}$ & 0.0021(5.6e-05)$^{\hspace{0.4em}}$ & 0.002(5.7e-05)$^{\hspace{0.4em}}$ & 0.0019(6e-05)$^{\hspace{0.4em}}$ & 0.002(8.8e-05)$^{\hspace{0.4em}}$ \\
359937 & black\_fr... & 3.5e+03(27)$^{\hspace{0.4em}}$ & 3.4e+03(30)$^{\hspace{0.4em}}$ & 3.4e+03(29)$^{\hspace{0.4em}}$ & 3.5e+03(31)$^{\hspace{0.4em}}$ & 3.4e+03(29)$^{\hspace{0.4em}}$ & 3.4e+03(27)$^{\hspace{0.4em}}$ & 3.4e+03(28)$^{\hspace{0.4em}}$ & 3.5e+03(32)$^{\hspace{0.4em}}$ \\
359938 & brazilia... & 1.2e+04(2e+04)$^{\hspace{0.4em}}$ & 1.5e+03(4.7e+03)$^{\hspace{0.4em}}$ & 1.4e+03(2.7e+03)$^{\hspace{0.4em}}$ & 4.6(4.9)$^{\hspace{0.4em}}$ & 2.7e+02(2e+02)$^{\hspace{0.4em}}$ & 3.9(5)$^{\hspace{0.4em}}$ & 1.9e+16(6.1e+16)$^{\hspace{0.4em}}$ & 4(5)$^{\hspace{0.4em}}$ \\
359939 & topo\_2\_1 & 0.028(0.0049)$^{\hspace{0.4em}}$ & 0.028(0.0049)$^{\hspace{0.4em}}$ & 0.028(0.0048)$^{\hspace{0.4em}}$ & 0.028(0.0048)$^{\hspace{0.4em}}$ & 0.028(0.0049)$^{\hspace{0.4em}}$ & 0.028(0.0049)$^{\hspace{0.4em}}$ & 0.028(0.0048)$^{\hspace{0.4em}}$ & 0.028(0.0049)$^{\hspace{0.4em}}$ \\
359940 & yprop\_4\_1 & 0.028(0.0049)$^{\hspace{0.4em}}$ & 0.028(0.0048)$^{\hspace{0.4em}}$ & 0.028(0.0049)$^{\hspace{0.4em}}$ & 0.028(0.0049)$^{\hspace{0.4em}}$ & 0.028(0.0049)$^{\hspace{0.4em}}$ & 0.028(0.0049)$^{\hspace{0.4em}}$ & 0.028(0.0049)$^{\hspace{0.4em}}$ & 0.028(0.0048)$^{\hspace{0.4em}}$ \\
359941 & onlinene... & 9.6e+05(3e+06)$^{\hspace{0.4em}}$ & 1.1e+04(3.7e+03)$^{1}$ & 1.1e+04(3.6e+03)$^{\hspace{0.4em}}$ & 3e+06(9.5e+06)$^{\hspace{0.4em}}$ & 1.1e+04(3.7e+03)$^{\hspace{0.4em}}$ & 1.1e+04(3.5e+03)$^{\hspace{0.4em}}$ & 1.1e+04(3.7e+03)$^{\hspace{0.4em}}$ & 1.1e+04(3.7e+03)$^{\hspace{0.4em}}$ \\
359942 & colleges & 0.13(0.0059)$^{\hspace{0.4em}}$ & 0.14(0.0057)$^{\hspace{0.4em}}$ & 0.14(0.0058)$^{\hspace{0.4em}}$ & 0.14(0.0052)$^{\hspace{0.4em}}$ & 0.14(0.0059)$^{\hspace{0.4em}}$ & 0.14(0.0053)$^{\hspace{0.4em}}$ & 0.14(0.006)$^{\hspace{0.4em}}$ & 0.14(0.0055)$^{\hspace{0.4em}}$ \\
359943 & nyc-taxi... & 1.5(0.15)$^{\hspace{0.4em}}$ & 1.8(0.15)$^{\hspace{0.4em}}$ & 1.6(0.15)$^{\hspace{0.4em}}$ & 1.8(0.18)$^{\hspace{0.4em}}$ & 1.7(0.16)$^{\hspace{0.4em}}$ & 1.7(0.18)$^{\hspace{0.4em}}$ & 1.6(0.18)$^{\hspace{0.4em}}$ & 1.8(0.17)$^{\hspace{0.4em}}$ \\
359944 & abalone & 2.1(0.12)$^{\hspace{0.4em}}$ & 2.1(0.11)$^{\hspace{0.4em}}$ & 2.1(0.12)$^{\hspace{0.4em}}$ & 2.1(0.1)$^{\hspace{0.4em}}$ & 2.1(0.1)$^{\hspace{0.4em}}$ & 2.1(0.12)$^{\hspace{0.4em}}$ & 2.1(0.12)$^{\hspace{0.4em}}$ & 2.1(0.11)$^{\hspace{0.4em}}$ \\
359945 & us\_crime & 0.13(0.0062)$^{\hspace{0.4em}}$ & 0.13(0.0065)$^{\hspace{0.4em}}$ & 0.13(0.0044)$^{\hspace{0.4em}}$ & 0.13(0.0065)$^{\hspace{0.4em}}$ & 0.13(0.007)$^{\hspace{0.4em}}$ & 0.13(0.0057)$^{\hspace{0.4em}}$ & 0.13(0.0062)$^{\hspace{0.4em}}$ & 0.13(0.0067)$^{\hspace{0.4em}}$ \\
359946 & pol & 2.7(0.29)$^{\hspace{0.4em}}$ & 3.8(0.54)$^{\hspace{0.4em}}$ & 3.7(0.36)$^{\hspace{0.4em}}$ & 3.9(0.22)$^{\hspace{0.4em}}$ & 3.3(0.45)$^{\hspace{0.4em}}$ & 3.9(0.31)$^{\hspace{0.4em}}$ & 2.3(0.26)$^{\hspace{0.4em}}$ & 4(0.31)$^{\hspace{0.4em}}$ \\
359948 & sat11-ha... & 8.8e+02(67)$^{\hspace{0.4em}}$ & 1.1e+03(66)$^{\hspace{0.4em}}$ & 1e+03(65)$^{\hspace{0.4em}}$ & 1.1e+03(61)$^{\hspace{0.4em}}$ & 9.5e+02(58)$^{\hspace{0.4em}}$ & 1.2e+03(1e+02)$^{\hspace{0.4em}}$ & 1e+03(95)$^{\hspace{0.4em}}$ & 1.1e+03(44)$^{\hspace{0.4em}}$ \\
359949 & house\_sa... & 1.1e+05(1.1e+04)$^{\hspace{0.4em}}$ & 1.2e+05(1.5e+04)$^{\hspace{0.4em}}$ & 1.1e+05(1.6e+04)$^{\hspace{0.4em}}$ & 1.1e+05(1.7e+04)$^{\hspace{0.4em}}$ & 1.1e+05(1.3e+04)$^{\hspace{0.4em}}$ & 1.1e+05(1.6e+04)$^{\hspace{0.4em}}$ & 1.1e+05(1.4e+04)$^{\hspace{0.4em}}$ & 1.2e+05(1.8e+04)$^{\hspace{0.4em}}$ \\
359950 & boston & 2.8(0.83)$^{\hspace{0.4em}}$ & 2.8(1)$^{\hspace{0.4em}}$ & 2.9(1)$^{\hspace{0.4em}}$ & 3.1(0.99)$^{\hspace{0.4em}}$ & 3(1.1)$^{\hspace{0.4em}}$ & 2.9(1)$^{\hspace{0.4em}}$ & 3(0.87)$^{\hspace{0.4em}}$ & 2.9(0.87)$^{\hspace{0.4em}}$ \\
359951 & house\_pr... & 2.4e+04(6.7e+03)$^{\hspace{0.4em}}$ & 2.6e+04(1e+04)$^{\hspace{0.4em}}$ & 2.5e+04(7.7e+03)$^{\hspace{0.4em}}$ & 2.5e+04(6.4e+03)$^{\hspace{0.4em}}$ & 2.8e+04(1.1e+04)$^{\hspace{0.4em}}$ & 2.5e+04(6.5e+03)$^{\hspace{0.4em}}$ & 2.5e+04(7e+03)$^{\hspace{0.4em}}$ & 2.9e+04(8.5e+03)$^{\hspace{0.4em}}$ \\
359952 & house\_16h & 2.8e+04(2.3e+03)$^{\hspace{0.4em}}$ & 3e+04(2.4e+03)$^{\hspace{0.4em}}$ & 3e+04(2e+03)$^{\hspace{0.4em}}$ & 3e+04(2e+03)$^{\hspace{0.4em}}$ & 2.9e+04(1.9e+03)$^{\hspace{0.4em}}$ & 2.9e+04(2.1e+03)$^{\hspace{0.4em}}$ & 2.9e+04(2e+03)$^{\hspace{0.4em}}$ & 3.1e+04(1.7e+03)$^{\hspace{0.4em}}$ \\
360932 & qsar-tid... & 0.72(0.072)$^{\hspace{0.4em}}$ & 0.77(0.067)$^{\hspace{0.4em}}$ & 0.72(0.071)$^{\hspace{0.4em}}$ & 0.75(0.066)$^{\hspace{0.4em}}$ & 0.73(0.071)$^{\hspace{0.4em}}$ & 0.73(0.068)$^{\hspace{0.4em}}$ & 0.71(0.052)$^{8}$ & 0.76(0.068)$^{\hspace{0.4em}}$ \\
360933 & qsar-tid... & 0.69(0.022)$^{\hspace{0.4em}}$ & 0.73(0.026)$^{\hspace{0.4em}}$ & 0.69(0.022)$^{\hspace{0.4em}}$ & 0.71(0.031)$^{\hspace{0.4em}}$ & 0.7(0.025)$^{\hspace{0.4em}}$ & 0.69(0.021)$^{\hspace{0.4em}}$ & 0.7(0.025)$^{\hspace{0.4em}}$ & 0.72(0.026)$^{\hspace{0.4em}}$ \\
360945 & mip-2016... & 2.1e+04(1.6e+03)$^{\hspace{0.4em}}$ & 2.2e+04(1.6e+03)$^{\hspace{0.4em}}$ & 2.1e+04(1.7e+03)$^{\hspace{0.4em}}$ & 2.1e+04(1.4e+03)$^{\hspace{0.4em}}$ & 2.1e+04(2.1e+03)$^{\hspace{0.4em}}$ & 2.1e+04(1.5e+03)$^{\hspace{0.4em}}$ & 2.2e+04(2e+03)$^{\hspace{0.4em}}$ & 2.2e+04(1.5e+03)$^{\hspace{0.4em}}$ \\
\bottomrule
\end{tabular}
\caption{Results for regression (in RMSE) on a one hour budget, denoted as \texttt{mean}(\texttt{std})$^{\mbox{\texttt{fails}}}$.}
\label{tab:neg_rmse-1h8c_gp3}
\end{table}
\end{landscape}
