# Supplementary material for: AMLB: an AutoML Benchmark
Source: arXiv:2207.12560 source file (2023-11-16)
Supplement: Supplementary file 7 [file neg_rmse-4h8c_gp3-table.tex]

\footnotesize
\begin{landscape}
\begin{table}
\tiny
\begin{tabular}{rlrrrrrrrr}
\toprule
 & framework& \unsizedsystemcase{autogluon}\ \ \  & \unsizedsystemcase{auto-sklearn}\ \ \ & \unsizedsystemcase{flaml}\ \ \ & \unsizedsystemcase{gama}\ \ \ & \unsizedsystemcase{h2o automl}\ \ \  & \unsizedsystemcase{light automl}\ \ \  & \unsizedsystemcase{mljar}\ \ \  & \unsizedsystemcase{tpot}\ \ \  \\
 task id & task name & & & & & & & & \\
\midrule
167210 & moneyball & 21(0.86)$^{\hspace{0.4em}}$ & 21(0.85)$^{\hspace{0.4em}}$ & 22(0.87)$^{\hspace{0.4em}}$ & 21(0.77)$^{\hspace{0.4em}}$ & 22(0.98)$^{\hspace{0.4em}}$ & 21(0.74)$^{\hspace{0.4em}}$ & 21(0.86)$^{\hspace{0.4em}}$ & 21(0.87)$^{\hspace{0.4em}}$ \\
233211 & diamonds & 5.1e+02(19)$^{\hspace{0.4em}}$ & 5.2e+02(19)$^{\hspace{0.4em}}$ & 5.2e+02(22)$^{1}$ & 5.2e+02(20)$^{\hspace{0.4em}}$ & 5.1e+02(19)$^{\hspace{0.4em}}$ & 5.2e+02(22)$^{\hspace{0.4em}}$ & 5.1e+02(22)$^{\hspace{0.4em}}$ & 5.3e+02(23)$^{\hspace{0.4em}}$ \\
233212 & allstate... & 1.9e+03(39)$^{\hspace{0.4em}}$ & 1.9e+03(58)$^{\hspace{0.4em}}$ & 1.9e+03(46)$^{\hspace{0.4em}}$ & 8.6e+12(2.7e+13)$^{\hspace{0.4em}}$ & 1.9e+03(47)$^{\hspace{0.4em}}$ & 1.9e+03(49)$^{\hspace{0.4em}}$ & 1.9e+03(60)$^{\hspace{0.4em}}$ & 1.9e+03(50)$^{\hspace{0.4em}}$ \\
233213 & buzzinso... & 1.5e+02(49)$^{\hspace{0.4em}}$ & 1.5e+02(50)$^{\hspace{0.4em}}$ & 1.5e+02(49)$^{\hspace{0.4em}}$ & 1.6e+02(47)$^{\hspace{0.4em}}$ & 1.5e+02(49)$^{\hspace{0.4em}}$ & 1.6e+02(45)$^{\hspace{0.4em}}$ & 1.5e+02(49)$^{\hspace{0.4em}}$ & 1.6e+02(46)$^{\hspace{0.4em}}$ \\
233214 & santande... & 6.8e+06(4.4e+05)$^{\hspace{0.4em}}$ & 6.8e+06(4.8e+05)$^{\hspace{0.4em}}$ & 6.8e+06(4.9e+05)$^{\hspace{0.4em}}$ & 6.9e+06(4.3e+05)$^{\hspace{0.4em}}$ & 6.9e+06(4.7e+05)$^{\hspace{0.4em}}$ & 6.9e+06(5.3e+05)$^{5}$ & 6.8e+06(4.6e+05)$^{\hspace{0.4em}}$ & 7e+06(4.4e+05)$^{\hspace{0.4em}}$ \\
233215 & mercedes... & 8.6(1)$^{\hspace{0.4em}}$ & 8.3(1.1)$^{\hspace{0.4em}}$ & 8.3(1.1)$^{\hspace{0.4em}}$ & 8.3(1.1)$^{\hspace{0.4em}}$ & 8.3(1.1)$^{\hspace{0.4em}}$ & 8.3(1.1)$^{\hspace{0.4em}}$ & 8.3(1.1)$^{\hspace{0.4em}}$ & 8.3(1.1)$^{\hspace{0.4em}}$ \\
317614 & yolanda & 8.3(0.043)$^{\hspace{0.4em}}$ & 8.7(0.051)$^{\hspace{0.4em}}$ & 8.6(0.06)$^{5}$ & 9.2(0.1)$^{\hspace{0.4em}}$ & 8.8(0.043)$^{\hspace{0.4em}}$ & 8.6(0.042)$^{\hspace{0.4em}}$ & 8.5(0.052)$^{\hspace{0.4em}}$ & 9.3(0.11)$^{\hspace{0.4em}}$ \\
359929 & airlines... & 29(0.24)$^{\hspace{0.4em}}$ & 29(0.28)$^{\hspace{0.4em}}$ & 29(0.21)$^{1}$ & 29(0.25)$^{\hspace{0.4em}}$ & 29(0.24)$^{\hspace{0.4em}}$ & 29(0.24)$^{\hspace{0.4em}}$ & 29(0.26)$^{1}$ & 29(0.28)$^{4}$ \\
359930 & quake & 0.19(0.0093)$^{\hspace{0.4em}}$ & 0.19(0.0089)$^{\hspace{0.4em}}$ & 0.19(0.0091)$^{\hspace{0.4em}}$ & 0.19(0.0092)$^{\hspace{0.4em}}$ & 0.19(0.0094)$^{\hspace{0.4em}}$ & 0.19(0.0099)$^{\hspace{0.4em}}$ & 0.19(0.0093)$^{\hspace{0.4em}}$ & 0.19(0.0096)$^{\hspace{0.4em}}$ \\
359931 & sensory & 0.67(0.061)$^{\hspace{0.4em}}$ & 0.69(0.051)$^{\hspace{0.4em}}$ & 0.69(0.054)$^{\hspace{0.4em}}$ & 0.68(0.055)$^{\hspace{0.4em}}$ & 0.7(0.062)$^{\hspace{0.4em}}$ & 0.69(0.061)$^{\hspace{0.4em}}$ & 0.67(0.043)$^{\hspace{0.4em}}$ & 0.68(0.054)$^{\hspace{0.4em}}$ \\
359932 & socmob & 12(8.9)$^{\hspace{0.4em}}$ & 11(3.5)$^{\hspace{0.4em}}$ & 15(8)$^{\hspace{0.4em}}$ & 14(7)$^{\hspace{0.4em}}$ & 14(13)$^{\hspace{0.4em}}$ & 19(9.3)$^{\hspace{0.4em}}$ & 20(29)$^{\hspace{0.4em}}$ & 16(8)$^{\hspace{0.4em}}$ \\
359933 & space\_ga & 0.094(0.013)$^{\hspace{0.4em}}$ & 0.1(0.025)$^{\hspace{0.4em}}$ & 0.1(0.015)$^{\hspace{0.4em}}$ & 0.096(0.019)$^{\hspace{0.4em}}$ & 0.097(0.012)$^{\hspace{0.4em}}$ & 0.1(0.017)$^{\hspace{0.4em}}$ & 0.099(0.018)$^{\hspace{0.4em}}$ & 0.099(0.018)$^{\hspace{0.4em}}$ \\
359934 & tecator & 0.83(0.18)$^{\hspace{0.4em}}$ & 0.76(0.34)$^{\hspace{0.4em}}$ & 0.85(0.17)$^{\hspace{0.4em}}$ & 0.82(0.33)$^{\hspace{0.4em}}$ & 0.82(0.3)$^{\hspace{0.4em}}$ & 0.79(0.26)$^{\hspace{0.4em}}$ & 0.85(0.19)$^{\hspace{0.4em}}$ & 0.56(0.094)$^{1}$ \\
359935 & wine\_qua... & 0.57(0.021)$^{\hspace{0.4em}}$ & 0.61(0.019)$^{\hspace{0.4em}}$ & 0.57(0.022)$^{\hspace{0.4em}}$ & 0.57(0.022)$^{\hspace{0.4em}}$ & 0.58(0.023)$^{\hspace{0.4em}}$ & 0.58(0.023)$^{\hspace{0.4em}}$ & 0.57(0.024)$^{\hspace{0.4em}}$ & 0.57(0.023)$^{\hspace{0.4em}}$ \\
359936 & elevators & 0.0018(5.2e-05)$^{\hspace{0.4em}}$ & 0.0019(7.3e-05)$^{\hspace{0.4em}}$ & 0.002(6.5e-05)$^{\hspace{0.4em}}$ & 0.0019(6.5e-05)$^{\hspace{0.4em}}$ & 0.002(0.00013)$^{\hspace{0.4em}}$ & 0.002(5.7e-05)$^{\hspace{0.4em}}$ & 0.0019(5.8e-05)$^{\hspace{0.4em}}$ & 0.0019(6.4e-05)$^{\hspace{0.4em}}$ \\
359937 & black\_fr... & 3.5e+03(28)$^{\hspace{0.4em}}$ & 3.4e+03(30)$^{\hspace{0.4em}}$ & 3.4e+03(27)$^{1}$ & 3.5e+03(29)$^{1}$ & 3.4e+03(30)$^{\hspace{0.4em}}$ & 3.4e+03(27)$^{\hspace{0.4em}}$ & 3.4e+03(29)$^{\hspace{0.4em}}$ & 3.5e+03(30)$^{\hspace{0.4em}}$ \\
359938 & brazilia... & 4.6e+04(1.2e+05)$^{\hspace{0.4em}}$ & 1.5e+03(4.7e+03)$^{\hspace{0.4em}}$ & 1.5e+03(2.7e+03)$^{\hspace{0.4em}}$ & 4.4(4.9)$^{\hspace{0.4em}}$ & 2.3e+02(2e+02)$^{\hspace{0.4em}}$ & 3.8(5)$^{\hspace{0.4em}}$ & 6.2e+14(2e+15)$^{\hspace{0.4em}}$ & 4.2(4.9)$^{\hspace{0.4em}}$ \\
359939 & topo\_2\_1 & 0.028(0.0049)$^{\hspace{0.4em}}$ & 0.028(0.0049)$^{\hspace{0.4em}}$ & 0.028(0.0048)$^{\hspace{0.4em}}$ & 0.028(0.0048)$^{\hspace{0.4em}}$ & 0.028(0.0049)$^{\hspace{0.4em}}$ & 0.028(0.0049)$^{\hspace{0.4em}}$ & 0.028(0.0048)$^{\hspace{0.4em}}$ & 0.028(0.0048)$^{\hspace{0.4em}}$ \\
359940 & yprop\_4\_1 & 0.028(0.0049)$^{\hspace{0.4em}}$ & 0.028(0.0048)$^{\hspace{0.4em}}$ & 0.028(0.0048)$^{\hspace{0.4em}}$ & 0.028(0.0049)$^{\hspace{0.4em}}$ & 0.028(0.0049)$^{\hspace{0.4em}}$ & 0.028(0.0049)$^{\hspace{0.4em}}$ & 0.028(0.0049)$^{\hspace{0.4em}}$ & 0.028(0.0048)$^{\hspace{0.4em}}$ \\
359941 & onlinene... & 4.3e+09(1.4e+10)$^{\hspace{0.4em}}$ & 1.1e+04(3.7e+03)$^{1}$ & 1.1e+04(3.8e+03)$^{1}$ & 1.1e+04(3.7e+03)$^{\hspace{0.4em}}$ & 1.2e+04(4.9e+03)$^{\hspace{0.4em}}$ & 1.1e+04(3.6e+03)$^{\hspace{0.4em}}$ & 1.3e+04(6e+03)$^{\hspace{0.4em}}$ & 1.1e+04(3.7e+03)$^{\hspace{0.4em}}$ \\
359942 & colleges & 0.13(0.0059)$^{\hspace{0.4em}}$ & 0.14(0.006)$^{\hspace{0.4em}}$ & 0.14(0.0061)$^{\hspace{0.4em}}$ & 0.14(0.0048)$^{\hspace{0.4em}}$ & 0.14(0.0055)$^{\hspace{0.4em}}$ & 0.14(0.0054)$^{\hspace{0.4em}}$ & 0.14(0.006)$^{\hspace{0.4em}}$ & 0.14(0.005)$^{\hspace{0.4em}}$ \\
359943 & nyc-taxi... & 1.6(0.14)$^{\hspace{0.4em}}$ & 1.6(0.23)$^{\hspace{0.4em}}$ & 1.6(0.044)$^{1}$ & 1.7(0.09)$^{6}$ & 1.6(0.15)$^{\hspace{0.4em}}$ & 1.7(0.17)$^{\hspace{0.4em}}$ & 1.6(0.14)$^{\hspace{0.4em}}$ & 1.8(0.16)$^{\hspace{0.4em}}$ \\
359944 & abalone & 2.1(0.12)$^{\hspace{0.4em}}$ & 2.1(0.11)$^{\hspace{0.4em}}$ & 2.1(0.12)$^{\hspace{0.4em}}$ & 2.1(0.1)$^{\hspace{0.4em}}$ & 2.1(0.11)$^{\hspace{0.4em}}$ & 2.1(0.12)$^{\hspace{0.4em}}$ & 2.1(0.12)$^{\hspace{0.4em}}$ & 2.1(0.11)$^{\hspace{0.4em}}$ \\
359945 & us\_crime & 0.13(0.0061)$^{\hspace{0.4em}}$ & 0.13(0.0066)$^{\hspace{0.4em}}$ & 0.13(0.0048)$^{\hspace{0.4em}}$ & 0.13(0.0059)$^{\hspace{0.4em}}$ & 0.13(0.0064)$^{\hspace{0.4em}}$ & 0.13(0.0059)$^{\hspace{0.4em}}$ & 0.13(0.0052)$^{\hspace{0.4em}}$ & 0.13(0.0058)$^{\hspace{0.4em}}$ \\
359946 & pol & 2.6(0.29)$^{\hspace{0.4em}}$ & 3.3(0.35)$^{\hspace{0.4em}}$ & 3.6(0.37)$^{\hspace{0.4em}}$ & 3.7(0.3)$^{\hspace{0.4em}}$ & 3.4(0.28)$^{\hspace{0.4em}}$ & 3.9(0.33)$^{\hspace{0.4em}}$ & 2.2(0.23)$^{\hspace{0.4em}}$ & 3.7(0.38)$^{\hspace{0.4em}}$ \\
359948 & sat11-ha... & 8.8e+02(67)$^{\hspace{0.4em}}$ & 1.1e+03(73)$^{\hspace{0.4em}}$ & 9.9e+02(63)$^{\hspace{0.4em}}$ & 1.1e+03(63)$^{\hspace{0.4em}}$ & 9.3e+02(63)$^{\hspace{0.4em}}$ & 1.2e+03(77)$^{\hspace{0.4em}}$ & 1.1e+03(1.1e+02)$^{\hspace{0.4em}}$ & 1e+03(69)$^{\hspace{0.4em}}$ \\
359949 & house\_sa... & 1.1e+05(1.1e+04)$^{\hspace{0.4em}}$ & 1.1e+05(1.4e+04)$^{\hspace{0.4em}}$ & 1.1e+05(1.8e+04)$^{\hspace{0.4em}}$ & 1.1e+05(1.6e+04)$^{\hspace{0.4em}}$ & 1.1e+05(1.2e+04)$^{\hspace{0.4em}}$ & 1.1e+05(1.6e+04)$^{\hspace{0.4em}}$ & 1.1e+05(1.2e+04)$^{\hspace{0.4em}}$ & 1.2e+05(1.2e+04)$^{\hspace{0.4em}}$ \\
359950 & boston & 2.8(0.83)$^{\hspace{0.4em}}$ & 2.9(1)$^{\hspace{0.4em}}$ & 2.8(0.62)$^{\hspace{0.4em}}$ & 3(0.99)$^{\hspace{0.4em}}$ & 2.8(0.81)$^{\hspace{0.4em}}$ & 2.9(1.1)$^{\hspace{0.4em}}$ & 3(0.93)$^{\hspace{0.4em}}$ & 3.1(1)$^{\hspace{0.4em}}$ \\
359951 & house\_pr... & 2.5e+04(7.6e+03)$^{\hspace{0.4em}}$ & 2.5e+04(9.4e+03)$^{\hspace{0.4em}}$ & 2.6e+04(7.7e+03)$^{\hspace{0.4em}}$ & 2.4e+04(5.9e+03)$^{\hspace{0.4em}}$ & 2.6e+04(8.5e+03)$^{\hspace{0.4em}}$ & 2.5e+04(6.8e+03)$^{\hspace{0.4em}}$ & 2.5e+04(7.1e+03)$^{\hspace{0.4em}}$ & 2.7e+04(7.8e+03)$^{\hspace{0.4em}}$ \\
359952 & house\_16h & 2.8e+04(2.3e+03)$^{\hspace{0.4em}}$ & 2.9e+04(2.4e+03)$^{\hspace{0.4em}}$ & 2.9e+04(2.1e+03)$^{\hspace{0.4em}}$ & 3e+04(2.2e+03)$^{\hspace{0.4em}}$ & 2.9e+04(1.9e+03)$^{\hspace{0.4em}}$ & 2.9e+04(2.1e+03)$^{\hspace{0.4em}}$ & 2.9e+04(2e+03)$^{\hspace{0.4em}}$ & 3.1e+04(2.1e+03)$^{\hspace{0.4em}}$ \\
360932 & qsar-tid... & 0.72(0.075)$^{\hspace{0.4em}}$ & 0.77(0.067)$^{\hspace{0.4em}}$ & 0.72(0.073)$^{\hspace{0.4em}}$ & 0.75(0.067)$^{\hspace{0.4em}}$ & 0.73(0.072)$^{\hspace{0.4em}}$ & 0.72(0.068)$^{\hspace{0.4em}}$ & 0.7(0.032)$^{5}$ & 0.74(0.069)$^{\hspace{0.4em}}$ \\
360933 & qsar-tid... & 0.69(0.022)$^{\hspace{0.4em}}$ & 0.73(0.033)$^{\hspace{0.4em}}$ & 0.68(0.023)$^{\hspace{0.4em}}$ & 0.71(0.025)$^{\hspace{0.4em}}$ & 0.69(0.023)$^{\hspace{0.4em}}$ & 0.69(0.021)$^{\hspace{0.4em}}$ & 0.7(0.022)$^{\hspace{0.4em}}$ & 0.71(0.027)$^{\hspace{0.4em}}$ \\
360945 & mip-2016... & 2.1e+04(1.6e+03)$^{\hspace{0.4em}}$ & 2.2e+04(1.6e+03)$^{\hspace{0.4em}}$ & 2.2e+04(1.5e+03)$^{\hspace{0.4em}}$ & 2.1e+04(1.4e+03)$^{\hspace{0.4em}}$ & 2.1e+04(1.9e+03)$^{\hspace{0.4em}}$ & 2.1e+04(1.5e+03)$^{\hspace{0.4em}}$ & 2.2e+04(1.4e+03)$^{\hspace{0.4em}}$ & 2.2e+04(2.2e+03)$^{\hspace{0.4em}}$ \\
\bottomrule
\end{tabular}
\caption{Results for regression (in RMSE) on a four hour budget, denoted as \texttt{mean}(\texttt{std})$^{\mbox{\texttt{fails}}}$.}
\label{tab:neg_rmse-4h8c_gp3}
\end{table}
\end{landscape}
