# Supplementary material for: AMLB: an AutoML Benchmark
Source: arXiv:2207.12560 source file (2023-11-16)
Supplement: Supplementary file 8 [file all-errors.tex]

\begin{table}
\caption{An overview of the types of errors aggregated over all frameworks.}
\begin{tabular}{lrrrrrrrrrr}
 & \multicolumn{2}{r}{framework} & \multicolumn{2}{r}{task} & \multicolumn{2}{r}{fold} & \multicolumn{2}{r}{constraint} & \multicolumn{2}{r}{info} \\
 & count & nunique & count & nunique & count & nunique & count & nunique & count & nunique \\
error &  &  &  &  &  &  &  &  &  &  \\
 & 2 & 2 & 2 & 2 & 2 & 2 & 2 & 2 & 2 & 2 \\
Data & 45 & 4 & 45 & 5 & 45 & 10 & 45 & 2 & 45 & 18 \\
Implementation & 274 & 3 & 274 & 27 & 274 & 10 & 274 & 2 & 274 & 64 \\
Memory & 287 & 8 & 287 & 27 & 287 & 10 & 287 & 2 & 287 & 30 \\
Timeout & 121 & 7 & 121 & 18 & 121 & 10 & 121 & 2 & 121 & 121 \\
\end{tabular}
\end{table}
