# Supplementary material for: AMLB: an AutoML Benchmark
Source: arXiv:2207.12560 source file (2023-11-16)
Supplement: Supplementary file 9 [file errors-per-subgroup-old.tex]

\begin{table}
\caption{An overview of the types of errors for frameworks starting with A-H. `tasks' denote how many unique tasks are affected, and `total' how frequent the error occurred in total.}
\begin{tabular}{lllrr}
 &  &  & tasks & total \\
framework & error & constraint &  &  \\
autogluon & Memory & 4h & 2 & 3 \\
\multirow{4}{*}{autosklearn} & \multirow{2}{*}{Data} & 1h & 1 & 1 \\
 &  & 4h & 1 & 1 \\
 & Memory & 1h & 1 & 1 \\
 & Timeout & 4h & 1 & 5 \\
autosklearn2 & Timeout & 4h & 1 & 10 \\
\multirow{4}{*}{flaml} &  & 4h & 1 & 1 \\
 & \multirow{2}{*}{Memory} & 1h & 4 & 18 \\
 &  & 4h & 16 & 58 \\
 & Timeout & 4h & 5 & 11 \\
\multirow{6}{*}{gama} & \multirow{2}{*}{Data} & 1h & 1 & 2 \\
 &  & 4h & 1 & 2 \\
 & \multirow{2}{*}{Implementation} & 1h & 4 & 26 \\
 &  & 4h & 4 & 28 \\
 & \multirow{2}{*}{Memory} & 1h & 2 & 9 \\
 &  & 4h & 7 & 32 \\
\end{tabular}
\end{table}


\begin{table}
\caption{An overview of the types of errors for frameworks starting with I-Z. `tasks' denote how many unique tasks are affected, and `total' how frequent the error occurred in total.}
\begin{tabular}{lllrr}
 &  &  & tasks & total \\
framework & error & constraint &  &  \\
\multirow{2}{*}{h2oautoml} & \multirow{2}{*}{Timeout} & 1h & 1 & 10 \\
 &  & 4h & 1 & 10 \\
\multirow{4}{*}{lightautoml} & \multirow{2}{*}{Memory} & 1h & 9 & 42 \\
 &  & 4h & 11 & 74 \\
 & \multirow{2}{*}{Timeout} & 1h & 2 & 2 \\
 &  & 4h & 2 & 2 \\
\multirow{8}{*}{mljarsupervised} &  & 1h & 1 & 1 \\
 & \multirow{2}{*}{Data} & 1h & 1 & 8 \\
 &  & 4h & 1 & 5 \\
 & \multirow{2}{*}{Implementation} & 1h & 14 & 72 \\
 &  & 4h & 15 & 118 \\
 & \multirow{2}{*}{Memory} & 1h & 1 & 7 \\
 &  & 4h & 2 & 9 \\
 & Timeout & 4h & 4 & 14 \\
\multirow{2}{*}{mlr3automl} & \multirow{2}{*}{Memory} & 1h & 2 & 13 \\
 &  & 4h & 2 & 20 \\
\multirow{7}{*}{tpot} & \multirow{2}{*}{Data} & 1h & 3 & 12 \\
 &  & 4h & 3 & 14 \\
 & \multirow{2}{*}{Implementation} & 1h & 7 & 16 \\
 &  & 4h & 6 & 14 \\
 & Memory & 4h & 1 & 1 \\
 & \multirow{2}{*}{Timeout} & 1h & 7 & 28 \\
 &  & 4h & 9 & 29 \\
\end{tabular}
\end{table}
